# Supplementary material for: Query Inseparability for ALC Ontologies
Source: arXiv:1902.00014 source file (2019-01-31)
Supplement: Supplementary file 1 [file appendix-2.tex]

%\documentclass[a4paper,11pt,twoside]{article}
%\documentclass{article}
%
%\usepackage{ijcai11}
%\usepackage{times}
%
%\usepackage{amsmath,amssymb,amsthm}
%\usepackage{epsfig}
%\usepackage{color}
%\usepackage{bbm}
%%\usepackage{boxedminipage}
%\usepackage{pifont}
%\usepackage{xspace}
%\usepackage{graphics}
%\usepackage{misc}
%\usepackage{url}

%\newcommand{\TWATA}{2ATA\xspace}
%\newcommand{\TWATAs}{2ATAs\xspace}
%\newcommand{\TWABA}{2ABTA\xspace}
%\newcommand{\TWABAs}{2ABTAs\xspace}

%\input{macros-def}
% %%%%%%%% Begin: Layout Instructions %%%%%%%%%%%%%%
% \hoffset -1in
% \voffset -1in
% \oddsidemargin 3.2cm
% \evensidemargin 3.3cm
% \headheight 2.5cm
% \textwidth14.6cm
% %\textwidth14.3cm
% \textheight21.5cm

% %%%%%%%% End: Layout Instructions %%%%%%%%%%%%%%%%

%\title{Foundations for Uniform Interpolation and Forgetting \\in Expressive Description Logics}
%\author{
  %\begin{tabular}[c]{ccc}
%Carsten Lutz &$\qquad$& Frank Wolter\\
%\textnormal{Fachbereich Informatik} && \textnormal{Department of Computer Science}\\
%\textnormal{Universit\"at Bremen, Germany} && \textnormal{University of Liverpool, UK}
%%wolter@liverpool.ac.uk}
  %\end{tabular}
%}
%
%\begin{document}
%
%\date{}
%%\maketitle
%
%

\section{Proof of Thereoms~\ref{thm:first} and \ref{thm:second}}

In this section we prove the semantic characterizations given in Theorem~\ref{thm:first} and
Theorem~\ref{thm:second}.
In what follows we assume that \hALC TBoxes are given in \emph{normal form} with concept inclusions
of the following form:
$$
A\sqsubseteq B, \quad A_{1} \sqcap A_{2} \sqsubseteq B, \quad \exists R.A \sqsubseteq B
$$
and
$$
A \sqsubseteq \bot, \quad \top \sqsubseteq B, \quad A \sqsubseteq \exists R.B, \quad A \sqsubseteq \forall R.B
$$
where $A,B$ range over concept names.
We define the canonical model $\I_{\T,\A}$ of a consistent \hALC KB $\K=(\T,\A)$ with $\T$ in normal form in the standard way using
a chase procedure. Consider the following rules that are applied to ABox $\Amc$:
\begin{enumerate}
\item if $A(a)\in \A$ and $A\sqsubseteq B\in\T$, then add $B(a)$ to $\A$;
\item if $A_{1}(a)\in A$ and $A_{2}(a)\in \A$ and $A_{1} \sqcap A_{2} \sqsubseteq B\in \T$, then add $B(a)$ to $\A$;
\item if $R(a,b)\in A$ and $A(b)\in \A$ and $\exists R.A \sqsubseteq B \in \T$, then add $B(a)$ to $\A$;
\item if $a\in {\sf ind}(\A)$ and $\top \sqsubseteq B\in \T$, then add $B(a)$ to $\A$;
\item if $A(a)\in \A$ and $A \sqsubseteq \exists R.B\in \T$ and there are no $R(a,b),B(b)\in \A$, then
add assertions $R(a,b),B(b)$ to $\A$ for a fresh $b$;
\item if $A(a)\in \A$ and $R(a,b)\in \A$ and $A \sqsubseteq \forall R.B\in \T$, then add $B(b)$ to $\A$.
\end{enumerate}
Denote by $\A^{c}$ the (possibly infinite) ABox resulting from $\A$ by applying these rules
exhaustively to $\A$. Then the canonical model $\I_{\T,\A}$ is the interpretation defined by $\A^c$.

\begin{theoremnum}{\ref{thm:second}}
Let $\Tmc_{1}$ and $\Tmc_{2}$ be \hALC TBoxes and $\Sigma_{1},\Sigma_{2}$ be
signatures.  Then $\Tmc_{1}$ $(\Sigma_{1},\Sigma_{2})$-CQ (equivalently,
$(\Sigma_{1},\Sigma_{2})$-UCQ) entails $\Tmc_{2}$ iff for all tree-shaped
$\Sigma_{1}$-ABoxes $\Amc$ of outdegree bounded by $|\Tmc_{2}|$ that are
consistent with $\Tmc_{1}$ and $\Tmc_{2}$, $\Imc_{\Tmc_{2},\Amc}$ is
$\Sigma_{2}$-homomorphically embeddable into $\Imc_{\Tmc_{1},\Amc}$.
\end{theoremnum}
\begin{proof}
The proof is similar to the proof of Theorem~\ref{thm:first}. Denote by $\mathcal{EL}^{u}$ the extension of $\mathcal{EL}$
with the universal role $u$.
Unravelling tolerance of \hALC implies also that if $(\T,\A)\models C(a)$ for a \hALC TBox $\T$ and $\mathcal{EL}^{u}$-concept $C$, then
$(\T,\A')\models C(a)$ for a finite subABox $\A'$ of the tree-unravelling $\A^{u}$ of $\A$ at $a$. Thus, any witness ABox for non-entailment
w.r.t.~$\mathcal{EL}^{u}$-instance queries can be transformed into a tree-shaped witness ABox. By the homomorphism criterion for $\Sigma$-CQ
entailment between \hALC-KBs proved in \cite{BotoevaKRWZ14} it is therefore sufficient to prove that if $\T_{1}$ does not $\Theta$-CQ-entail $\T_{2}$, then
this is witnessed by an $\mathcal{EL}^{u}$-instance query $C(a)$. This proof is a straightforward extension of the proof of Theorem~\ref{thm:first}.
\end{proof}

The notion of con-$\Sigmaquery$-homomorphic embeddability is slightly
unwieldy to use in the subsequent definitions and constructions. We
therefore resort to simulations. % , introduced next.  Let $\Imc_1,\Imc_2$
% be interpretations and $\Sigma$ a signature.  A relation $S\subseteq
% \Delta^{\Imc}\times \Delta^{\Imc}$ is a \emph{$\Sigma$-simulation}
% from $\Imc_{1}$ to $\Imc_{2}$ if
% \begin{itemize}
% \item $(d,d')\in S$ and $d\in  A^{\Imc_{1}}$ implies $d'\in
%   A^{\Imc_{2}}$ for all $\Sigma$-concept names $A$;
% \item $(d,d')\in S$ and $(d,e)\in R^{\Imc_{1}}$ implies that there is
%   a $(d',e')\in R^{\Imc_{2}}$ such that $(e,e')\in S$  for all
%   $\Sigma$-role names~$R$.
% \end{itemize}
% %
% Let $d_i \in \Delta^{\Imc_i}$, $i \in \{1,2\}$.
% $(\Imc_{1},d_{1})$ is $\Sigma$-simulated by $(\Imc_{2},d_{2})$,
% in symbols $(\Imc_{1},d_{1}) \leq_{\Sigma}(\Imc_{2},d_{2})$, if
% there exists a $\Sigma$-simulation $S$ with $(d_{1},d_{2})\in S$.
%
The following lemma gives an analysis of
non-con-$\Sigmaquery$-homomorphic embeddability in terms of
simulations that is relevant for the subsequent constructions.
%
% otherwise, we would have to go to sigma-connected sub-interpretations
%

\begin{lemmanum}{\ref{lem:homtosim}}
  % Let \Amc be a $\Sigmaabox$-ABox and $\Imc_1$ a model of $(\Tmc_1,\Amc)$ and
  % $\Imc_2$ a forest-shaped model of $(\Tmc_2,\Amc)$. Then $\Imc_2$ is not
  % con-$\Sigmaquery$-homomorphically embeddable into $\Imc_1$ iff there is an $a
  % \in \mn{ind}(\Amc)$ such that one of the following is true:
  % %
  % \begin{enumerate}
  %
  % \item there is a $\Sigmaquery$-concept name $A$ with
  %   $a \in A^{\Imc_2} \setminus A^{\Imc_1}$;
  %
  % \item there is an $R_0$-successor $d_0$ of $a$ in
  %   $\Imc_{2}$, for some $\Sigmaquery$-role name $R_0$, such
  %   that $d_0 \notin \mn{ind}(\Amc)$ and for all $R_0$-successors $d$
  %   of $a$ in $\Imc_1$, we have that $(\Imc_{2},d_0)
  %   \not\leq_{\Sigmaquery}(\Imc_1,d)$.
  %
  % \end{enumerate}
Let \Amc be a $\Sigmaabox$-ABox and $\Imc_1$ a model of $(\Tmc_1,\Amc)$. Then
$\Imc_{\Tmc_2,\Amc}$ is not con-$\Sigmaquery$-homomorphically embeddable into
$\Imc_1$ iff there is $a \in \mn{ind}(\Amc)$ such that one of the following
holds:
  \begin{enumerate}\itemsep 0cm

  \item[\rm (1)] there is a $\Sigmaquery$-concept name $A$ with
    $a \in A^{\Imc_{\Tmc_2,\Amc}} \setminus A^{\Imc_1}$;

  \item[\rm (2)] there is an $R$-successor $d$ of $a$ in
    $\Imc_{\Tmc_2,\Amc}$, for some $\Sigmaquery$-role name $R$, such
    that $d \notin \mn{ind}(\Amc)$ and, for all $R$-successors $e$
    of $a$ in $\Imc_1$, we have  $(\Imc_{\Tmc_2,\Amc},d)
    \not\leq_{\Sigmaquery}(\Imc_1,e)$.

  \end{enumerate}
\end{lemmanum}
\begin{proof}(sketch) The ``if'' direction is clear by definition of
  homomorphisms and because of the following: if there is a
  $\Sigmaquery$-homomorphism $h$ from the maximal $\Sigma$-connected
  subinterpretation of $\Imc_{\Tmc_2,\Amc}$ to $\Imc_1$, $a \in
  \mn{ind}(\Amc)$, and $d$ is an $R$-successor of $a$ in $\Imc_{\Tmc_2,\Amc}$ with $R
  \in \Sigmaquery$ and $d \notin \mn{ind}(\Amc)$, then $h(d)$ is an
  $R$-successor of $a$ in $\Imc_1$ and $h$ contains a
  $\Sigmaquery$-simulation from $(\Imc_{\Tmc_2,\Amc},d)$ to $(\Imc_1,h(d))$.

  For the ``only if'' direction, assume that both Point~1 and Point~2 are false
  for all $a \in \mn{ind}(\Amc)$. Then for every $a \in \mn{ind}(\Amc)$,
  $R$-successor $d$ of $a$ in $\Imc_{\Tmc_2,\Amc}$ with $R \in \Sigmaquery$ and
  $d \notin \mn{ind}(\Amc)$, there is an $R$-successor $d'$ of $a$ in $\Imc_1$
  and a simulation $\S_d$ from $\Imc_1$ to $\Imc_{\Tmc_2,\Amc}$ such that
  $(d,d') \in \S_d$. Because the subinterpretation of $\Imc_{\Tmc_2,\Amc}$ rooted at $d$ is
  tree-shaped, we can assume that $\S_d$ is a partial function. Now consider
  the function $h$ defined by setting $h(a)=a$ for all $a \in \mn{ind}(\Amc)$
  and then taking the union with all the simulations $\S_d$. It can be verified
  that $h$ is a $\Sigmaquery$-homomorphism from the maximal $\Sigma$-connected
  subinterpretation of $\Imc_{\Tmc_2,\Amc}$ to $\Imc_1$.
\end{proof}

\section{Proof of Theorem~\ref{thm:exptbox}}

We aim to prove Theorem~\ref{thm:exptbox}, i.e., that it is \ExpTime-complete
to decide whether an \ALC TBox $\Tmc_1$ $(\Sigma_1,\Sigma_2)$-\RCQ entails a
Horn-\ALC TBox $\Tmc_2$. We are going to use automata on finite trees.

\subsection{Tree Automata Preliminaries}

We introduce two-way alternating B\"uchi automata on finite trees
(\TWABAs).  A finite tree $T$ is \emph{$m$-ary} if for every $x \in T$,
the set $\{ i \mid x \cdot i \in T \}$ is of cardinality zero or
exactly $m$.  An \emph{infinite path} $P$ of $T$ is a prefix-closed
set $P \subseteq T$ such that for every $i \geq 0$, there is a unique
$x \in P$ with $|x|=i$.
\begin{definition}[\TWABA]
  A \emph{two-way alternating B\"uchi automaton (\TWABA) on finite
    $m$-ary trees} is a tuple $\Amf=(Q,\Gamma,\delta,q_0,R)$ where $Q$
  is a finite set of \emph{states}, $\Gamma$ is a finite alphabet,
  $\delta: Q \times \Gamma \rightarrow \Bmc^+(\mn{tran}(\Amf))$ is the
  \emph{transition function} with $\mn{tran}(\Amf) = ([m] \times Q)
  \cup \mn{leaf}$ the set of \emph{transitions} of \Amf, $q_0 \in Q$
  is the \emph{initial state}, and $R \subseteq Q$ is a set of
  \emph{recurring states}.
\end{definition}
Transitions have the same intuition as for \TWATAs on infinite trees.
The additional transition $\mn{leaf}$ verifies that the automaton is
currently at a leaf node.
\begin{definition}[Run, Acceptance]
  A \emph{run} of a \TWABA $\Amf = (Q,\Gamma,\delta,q_0,R)$ on a finite
  $\Gamma$-labeled tree $(T,L)$ is a $T \times Q$-labeled tree
  $(T_r,r)$ such that the following conditions are satisfied:
  \begin{enumerate}

  \item $r(\varepsilon) = ( \varepsilon, q_0)$

  \item if $y \in T_r$, $r(y)=(x,q)$, and $\delta(q,L(x))=\vp$, then
    there is a (possibly empty) set $Q = \{ (c_1,q_1),\dots,(c_n,q_n)
    \} \subseteq \mn{tran}(\Amf)$ such that $Q$ satisfies $\vp$ and
    for $1 \leq i \leq n$, $x \cdot c_i$ is defined and  a node
    in $T$, and there is a $y \cdot i \in T_r$ such that $r(y \cdot
    i)=(x \cdot c_i,q_i)$;

  \item if $r(y)=(x,\mn{leaf})$, then $x$ is a leaf in $T$.

  \end{enumerate}
  We say that $(T_r,r)$ is \emph{accepting} if in all infinite paths
  $\varepsilon = y_1 y_2 \cdots$ of $T_r$, the set $\{ i \geq 0 \mid
  r(y_i)=(x,q) \text{ for some } q \in R\}$ is infinite.\nb{E: is it really
    like this? shouldn't it be that only the states in $R$ are allowed to
    appear infinitely often?}
  A finite $\Gamma$-labeled tree $(T,L)$ is \emph{accepted} by \Amf if
  there is an accepting run of \Amf on $(T,L)$. We use $L(\Amf)$ to
  denote the set of all finite $\Gamma$-labeled tree accepted by \Amf.
\end{definition}
Apart from \TWABAs,
we will also use nondeterministic tree automata, introduced next.
\smallskip

A \emph{nondeterministic top-down tree automaton} (NTA) on finite
$m$-ary trees is a tuple $\Amf=(Q, \Gamma, Q^0, \delta, F)$ where $Q$
is a finite set of \emph{states}, $\Gamma$ is a finite alphabet, $Q^0
\subseteq Q$ is the set of \emph{initial states}, $F \subseteq Q$ is a
set of \emph{final states}, and $\delta:Q \times \Gamma
\rightarrow 2^{Q^m}$ is the \emph{transition function}.

Let $(T,L)$ be a $\Gamma$-labeled $m$-ary tree.  A \emph{run} of \Amf
on $(T,L)$ is a $Q$-labeled $m$-ary tree $(T,r)$ such that
$r(\varepsilon) \in Q^0$ and for each node $x \in T$, we have $\langle
r(x \cdot 1), \ldots ,r(x \cdot m)\rangle \in \delta( r(x),
L(x))$. The run is \emph{accepting} if for every leaf $x$ of $T$, we
have $r(x) \in F$. The set of trees accepted by $\mathcal A$ is
denoted by $L(\mathcal A)$.

We will use the following results from automata theory:
\begin{theorem}~\\[-4mm]
  \begin{enumerate}

  \item Every \TWABA $\Amf=(Q,\Gamma,\delta,q_0,R)$ can be converted
    into an equivalent NTA $\Amf'$ whose number of states is (single)
    exponential in $|Q|$; the conversion needs time polynomial in the
    size of $\Amf'$;

  \item Given a constant number of \TWABAs (resp.\ NTAs), we can
    construct in polytime a \TWABA (resp.\ an NTA) that accepts the
    intersection language;

  \item Emptiness of NTAs can be checked in polytime.

  \end{enumerate}
\end{theorem}

\subsection{$\Gamma$-labeled Trees}

For the proof of Theorem~\ref{thm:exptbox}, fix an \ALC TBox $\Tmc_1$ and a
Horn-\ALC TBox~$\Tmc_2$ and signatures $\Sigmaabox,\Sigmaquery$.  Set $m :=
|\Tmc_2|$.  Ultimately, we aim to construct an NTA \Amf such that a tree is
accepted by \Amf if and only if this tree encodes a $\Sigmaabox$-ABox \Amc of
outdegree at most $m$ that is consistent with both $\Tmc_1$ and $\Tmc_2$ and a
model $\Imc_1$ of $(\Tmc_1,\Amc)$ such that the canonical model
$\Imc_{\Tmc_2,\Amc}$ of $(\Tmc_2,\Amc)$ is not
con-$\Sigmaquery$-homomorphically embeddable into $\Imc_1$.  By
Theorem~\ref{thm:first}, this means that \Amf accepts the empty language if and
only if $\Tmc_2$ is $(\Sigma_1,\Sigma_2)$-rCQ entailed by $\Tmc_1$.  In this
section, we make precise which trees should be accepted by the NTA \Amf and in
the subsequent section, we construct \Amf.

As before, we assume that $\Tmc_1$ takes the form $\top \sqsubseteq C_{\T_1}$
with $C_{T_1}$ in NNF and use $\mathsf{cl}(C_{\T_1})$ to denote the set of
subconcepts of $C_{\T_1}$, closed under single negation.
We also assume that $\Tmc_2$ is in the Horn-\ALC normal form introduced
above. We use $\mn{CN}(\Tmc_2)$ to denote the
set of concept names in $\Tmc_2$ and $\mn{sub}(\Tmc_2)$ for the set of
subconcepts of (concepts in) $\Tmc_2$.

Let $\Gamma_0$ denote the set of all subsets of
$\Sigmaabox \cup \{ R^- \mid R \in \Sigmaabox \}$ that contain at most one
role.  Automata will run on $m$-ary $\Gamma$-labeled trees where
$$
\Gamma = \Gamma_0 \times 2^{\mn{cl}(\Tmc_1)} \times 2^{\mn{CN}(\Tmc_2)}
\times \{ 0,1 \} \times 2^{\mn{sub}(\Tmc_2)}.
$$
For easier reference, in a $\Gamma$-labeled tree $(T,L)$ and for a node $x$
from $T$, we write $L_i(x)$ to denote the $i+1$st component of $L(x)$, for each
$i \in \{0,\dots,4\}$. Intuitively, the projection of a $\Gamma$-labeled tree
to
\begin{itemize}

\item the $L_0$-components of its $\Gamma$-labels represents the
  $\Sigmaabox$-ABox \Amc that witnesses non-$\Sigmaquery$-query
  entailment of $\Tmc_2$ by $\Tmc_1$;

\item $L_1$-components (partially) represents a model $\Imc_1$ of
  $(\Tmc_1,\Amc)$;

\item $L_2$-components (partially) represents the
  canonical model $\Imc_{\Tmc_2,\Amc}$ of $(\Tmc_2,\Amc)$;

\item $L_3$-components marks the individual $a$ in \Amc such that
  $(\Imc_{\Tmc_2,\Amc},a)$ is not $\Sigmaquery$-simulated by
  $(\Imc_{\Tmc_1,\Amc},a)$;

\item $L_4$-components contains bookkeeping information that helps to
  ensure that the afore mentioned $\Sigmaquery$-simulation indeed fails.

\end{itemize}
We now make these intuitions more precise by defining certain
properness conditions for $\Gamma$-labeled trees, one for each
component in the labels.  A $\Gamma$-labeled $(T,L)$ tree is
\emph{0-proper} if
%$L_0(\varepsilon)$ contains no role.
it satisfies the following conditions:
\begin{enumerate}

\item for the root $\varepsilon$ of $T$, $L_0(\varepsilon)$ contains no role;

\item every non-root node $x$ of $T$, $L_0(x)$ contains a role.

\end{enumerate}
Every 0-proper $\Gamma$-labeled tree $(T, L)$ represents the
tree-shaped $\Sigmaabox$-ABox
\begin{align*}
\Amc_{( T, L)} = \ & \{ A(x) \mid A \in L_0(x) \}\\[1mm] % \cap \NC  \}\\
  & \cup \{ R(x,y) \mid R \in L_0(y), y \text{ is a child of } x \}\\  %last item ensure x not the root
  & \cup \{ R(y,x) \mid  R^{-} \in L_0(y), y \text{ is a child of } x \}. % same here, x not root
\end{align*}
A $\Gamma$-labeled tree $(T, L)$ is \emph{1-proper} if it
satisfies the following conditions for all $x_1,x_2 \in T$:
\begin{enumerate}

\item there is a model \Imc of $\Tmc_1$ and a $d \in \Delta^\Imc$ such
  that $d \in C^\Imc$ iff $C \in L_1(x_1)$ for all $C \in
  \mn{cl}(\Tmc_1)$;

%\item for every node $x$, $L_1(x)=\mn{cl}_\Tmc(L_1(x))$;

\item $A \in L_0(x_1)$ implies $A \in L_1(x_1)$;

\item if $x_2$ is a child of $x_1$ and $R \in x_2$, then $\forall R . C
  \in L_1(x_1)$ implies $C \in L_1(x_2)$ for all $\forall R . C \in \mn{cl}(\Tmc_1)$;

\item if $x_2$ is a child of $x_1$ and $R^- \in x_2$, then $\forall R . C
  \in L_1(x_2)$ implies $C \in L_1(x_1)$ for all $\forall R . C \in \mn{cl}(\Tmc_1)$.

\end{enumerate}
A $\Gamma$-labeled tree $(T, L)$ is \emph{2-proper} if for every node
$x \in T$,
\begin{enumerate}

\item  $A \in L_2(x)$ iff $\Amc_{(T,L)},\Tmc_2 \models A(x)$, for all $A
  \in \mn{CN}(\Tmc_2)$;

\item if $A \in L_2(x)$, then $A \sqsubseteq \bot \notin \Tmc_2$.

% \item \emph{3-proper} if there is exactly one node $x$ with
%   $L_3(x)=1$.

\end{enumerate}
%
%A $\Gamma$-labeled tree $(T, L)$
It is \emph{3-proper} if there is
exactly one node $x$ with $L_3(x)=1$.  For defining 4-properness,
we first give some preliminaries.

Let $t \subseteq \mn{CN}(\Tmc_2)$. Then $\mn{cl}_{\Tmc_2(S)} = \{ A \in
\mn{CN}(\Tmc_2) \mid \Tmc_2 \models \midsqcap S \sqsubseteq A \}$. Moreover, we
say that $S = \{ \exists R . A, \forall R . B_1, \dots, \forall R . B_n \}$ is
a \emph{$\Sigmaquery$-successor set for} $t$ if there is
a %role name $r \in \Sigmaquery$ and a
concept name $A' \in t$ such that $A' \sqsubseteq \exists R . A \in \Tmc_2$ and
$\forall R . B_1, \dots, \forall R . B_n$ is the set of all concepts of this
form such that, for some $B \in t$, we have $B \sqsubseteq \forall R . B_i \in
\Tmc_2$. In the following, it will sometimes be convenient to speak about the
canonical model $\Imc_{\Tmc_2,\Smc}$ of $\Tmc_2$ and a finite set of concepts
$C$ that occur on the right-hand side of a CI in $\Tmc_2$. What we mean with
$\Imc_{\Tmc_2,\Smc}$ is the interpretation obtained from the canonical model
for the TBox $\Tmc_i \cup \{ A_C \sqsubseteq C \mid C \in \Smc \}$ and the ABox
$ \{ A_C(a_\varepsilon) \mid C \in \Smc \}$ in which all fresh concept names
$A_C$ are removed.

A $\Gamma$-labeled tree is \emph{4-proper} if it satisfies the
following conditions for all nodes $x_1$, $x_2$:
\begin{enumerate}

\item if $L_3(x_1)=1$, then there is a $\Sigmaquery$-concept name in $L_2(x_1)
  \setminus L_1(x_1)$ or $L_4(x_1)$ is
% a set
%   %
%   $$
%     \{ \exists r . C, \forall r . D_1, \cdots \forall r . D_n \}
%   $$
%   %
%   such that {\color{blue} $\Tmc \models L_2(x) \sqsubseteq \exists u . \midsqcap
%   L_4(x)$;}
a $\Sigmaquery$-successor set for~$L_2(x_1)$;

\item if $L_4(x_1) \neq \emptyset$, then there is a model \Imc of
  $\Tmc_1$ and a $d \in \Delta^\Imc$ such that $d \in C^\Imc$ iff $C
  \in L_1(x_1)$ for all $C \in \mn{cl}(\Tmc_1)$ and
  $(\Imc_{\Tmc_2,L_4(x_1)},a_\varepsilon) \not\leq_{\Sigmaquery} (\Imc,d)$;

% \item if $L_3(x) \neq \emptyset$, then for all successor sets $S$ from
%   $L_1(x)$, there is {\color{blue}no $\Sigma$-simulation from
%     $\Imc_{\Tmc_2,L_3(x)}$ to
%     $\Imc_{\Tmc_1,S}$;\footnote{\color{blue}here and elsewhere: fix
%       notation}} {\color{red}CANONICAL!!!}

\item if $x_2$ is a child of $x_1$, $L_0(x_2)$ contains the role name
  $R$, and $L_4(x_1)= \{ \exists R . A, \forall R . B_1, \dots,\forall
  R . B_n \}$, then
  %
%  \begin{enumerate}
%  \item
there is a $\Sigmaquery$-concept name in
  $\mn{cl}_{\Tmc_2}(\{A,B_1,\dots,B_n\}) \setminus L_1(x_2)$ or
%  \item
$L_4(x_2)$ is
  a $\Sigmaquery$-successor set for $\mn{cl}_{\Tmc_2}(\{A,B_1,\dots,B_n\})$;
%  \end{enumerate}

\item if $x_2$ is a child of $x_1$, $L_0(x_2)$ contains the role
  $R^-$, and $L_4(x_2)= \{ \exists R . A, \forall R . B_1,
  \dots,\forall R . B_n \}$, then
  %
%  \begin{enumerate}
%
%  \item
there is a $\Sigmaquery$-concept name in
  $\mn{cl}_{\Tmc_2}(\{A,B_1,\dots,B_n\}) \setminus L_1(x_1)$ or
%
 % \item
$L_4(x_1)$ is
  a $\Sigmaquery$-successor set for $\mn{cl}_{\Tmc_2}(\{A,B_1,\dots,B_n\})$.
%  \end{enumerate}
%

% \item if $L_4(x_1)=\{ \exists r . A, \forall r . B_1,\dots, \forall r
%   . B_n \}$, then $x_1$ has an $r$-successor in $\Amc_{(T,L)}$.

\end{enumerate}
Note how 4-properness addresses Condition~2 of
Lemma~\ref{lem:homtosim}. By that condition, there is a set of
simulations from certain pointed ``source'' interpretations to
certain pointed ``target'' interpretations that should be avoided.
In the $L_4$-component of $\Gamma$-labels, we store the source
interpretations, represented as sets of concepts. 4-properness
then ensures that there is no simulation to the relevant target
interpretations.
\begin{lemma}
\label{lem:gammattrees}
  % $\Tmc_1$ does not $\Sigmaquery$-CQ entail $\Tmc_2$ iff there is an
  % $m$-ary $\Gamma$-labeled tree that is $i$-proper for all $i \in
  % \{0,\dots,4\}$.
There is an $m$-ary $\Gamma$-labeled tree that is $i$-proper for all
$i \in \{0,\dots,4\}$ iff there is a tree-shaped $\Sigmaabox$-ABox
$\Amc$ of outdegree at most $m$ that is consistent w.r.t.\ $\Tmc_1$
and $\Tmc_2$ and a model $\Imc_1$ of
$(\Tmc_1,\Amc)$ such that the canonical model $\Imc_{\Tmc_2,\Amc}$ of
$(\Tmc_2,\Amc)$ is not con-$\Sigmaquery$-homomorphically embeddable
into $\Imc_1$.
\end{lemma}
\begin{proof}
  ``if''. Let $(T,L)$ be an $m$-ary $\Gamma$-labeled tree that is
  $i$-proper for all $i \in \{0,\dots,4\}$. Then $\Amc_{(T,L)}$ is a
  tree-shaped $\Sigmaabox$-ABox of outdegree at most $m$.  Moreover,
  $\Amc_{(T,L)}$ is consistent w.r.t.\ $\Tmc_2$: because of the second
  condition of 2-properness, the canonical model $\Imc_{\Tmc_2,\Amc}$
  of $(\Tmc_2,\Amc)$ is indeed a model of $\Tmc_2$ and \Amc.

  Since $(T,L)$ is $3$-proper, there is exactly one $x_0 \in T$ with
  $L_3(x_0)=1$. By construction, $x_0$ is also an individual name in
  $\Amc_{(T,L)}$.  To finish this direction of the proof, it suffices
  to construct a model $\Imc_1$ of $(\Tmc_1,\Amc_{(T,L)})$ such that
  $(\Imc_{\Tmc_2,\Amc},x_0) \not\leq_{\Sigmaquery} (\Imc_1,x_0)$.  In
  fact, $\Imc_1$ witnesses consistency of $\Amc_{(T,L)}$ with
  $\Tmc_1$. Moreover, by definition of simulations $\Imc_1$ must
  satisfy one of Points~1 and~2 of Lemma~\ref{lem:homtosim} with $a$
  replaced by $x_0$. Consequently, by that Lemma $\Imc_{\Tmc_2,\Amc}$
  is not con-$\Sigmaquery$-homomorphically embeddable into $\Imc_1$.

  Start with the interpretation $\Imc_0$ defined as follows:
  $$
  \begin{array}{r@{~}c@{~}l}
    \Delta^{\Imc_0} &=& T \\[1mm]
    A^{\Imc_0} &=& \{ x \in T \mid A \in L_1(x) \} \\[1mm]
    R^{\Imc_0} &=& \{ (x_1,x_2) \mid x_2 \text{ child of } x_1 \text{
                   and } R \in L_0(x_2) \} \, \cup{} \\[1mm]
    && \{ (x_2,x_1) \mid x_2 \text{ child of } x_1 \text{
                   and } R^- \in L_0(x_2) \}.
  \end{array}
  $$
  Then take, for each $x \in T$, a model $\Imc_x$ of \Tmc such that
  $x \in C^{\Imc_x}$ iff $C \in L_1(x)$ for all
  $C \in \mn{cl}(\Tmc_1)$.  Moreover, if $L_4(x) \neq \emptyset$,
  then choose $\Imc_x$ such that $(\Imc_{\Tmc_2,L_3(x)},a_\varepsilon)
  \not\leq_{\Sigmaquery} (\Imc_x,x)$. These choices are possible since $(T,L)$ is 1-proper
  and 4-proper. Further assume that $\Delta^{\Imc_0}$ and
  $\Delta^{\Imc_x}$ share only the element $x$. Then $\Imc_1$ is the
  union of $\Imc_0$ and all chosen interpretations $\Imc_x$.  It is
  not difficult to prove that $\Imc_1$ is indeed a model of
  $(\Tmc_1,\Amc_{(T,L)})$.

  We show that $(\Imc_{\Tmc_2,\Amc_{(T,L)}},x_0)
  \not\leq_{\Sigmaquery} (\Imc_1,x_0)$.
  By Point~1 of 4-properness, there is a $\Sigmaquery$-concept name in
  $L_2(x_0) \setminus L_1(x_0)$ or $L_4(x_0)$ is a
  $\Sigmaquery$-successor set for $L_2(x)$. In the former case, we are
  done. In the latter case, it suffices to show the following.
  \\[2mm]
  {\bf Claim.} For all $x \in T$: if $L_4(x) \neq \emptyset$, then
    $(\Imc_{\Tmc_2,L_4(x)},a_\varepsilon) \not\leq_{\Sigmaquery}(\Imc_1,x)$.
  \\[2mm]
  The proof of the claim is by induction on the co-depth of $x$ in
  $\Amc_{(T,L)}$, which is the length $n$ of the longest sequence of
  role assertions $R_1(x,x_1),\dots,R_n(x_{n-1},x_n)$ in
  $\Amc_{(T,L)}$. It uses Conditions~2 to~4 of 4-properness.

  \medskip

  ``only if''. Let \Amc be a $\Sigmaabox$-ABox of outdegree at most $m$ that is
  consistent w.r.t.\ $\Tmc_1$ and $\Tmc_2$, and $\Imc_1$ a model of
  $(\Tmc_1,\Amc)$ such that $\Imc_{\Tmc_2,\Amc}$ is not
  con-$\Sigmaquery$-homomorphically embeddable into $\Imc_1$. By duplicating
  successors, we can make sure that every non-leaf in \Amc has exactly $m$
  successors. We can further assume w.l.o.g.\ that $\mn{ind}(\Amc)$ is a
  prefix-closed subset of $\mathbbm{N}^*$ that reflects the tree-shape of \Amc,
  that is, $R(a,b) \in \Amc$ implies $b=a\cdot c$ or $a = b \cdot c$ for some
  $c \in \mathbbm{N}$.  By Lemma~\ref{lem:homtosim}, there is an $a_0 \in
  \mn{ind}(\Amc)$ such that one of the following holds:
  \begin{enumerate}

  \item there is a $\Sigmaquery$-concept name $A$ with
    $a_0 \in A^{\Imc_{\Tmc_2,\Amc}} \setminus A^{\Imc_1}$;

  \item there is an $R_0$-successor $d_0$ of $a_0$ in
    $\Imc_{\Tmc_2,\Amc}$, for some $\Sigmaquery$-role name $R_0$, such
    that $d_0 \notin \mn{ind}(\Amc)$ and for all $R_0$-successors $d$
    of $a_0$ in $\Imc_1$, we have that $(\Imc_{\Tmc_2,\Amc},d_0)
    \not\leq_{\Sigmaquery}(\Imc_1,d)$.

  \end{enumerate}
  We now show how to construct from \Amc a $\Gamma$-labeled tree
  $(T,L)$ that is $i$-proper for all $i \in \{0,\dots,4 \}$.  For each
  $a \in \mn{ind}(\Amc)$, let $R(a)$ be undefined if $a=\varepsilon$
  and otherwise let $R(a)$ be the unique role $R$ (i.e., role name or
  inverse role) such that $R(b,a) \in \Amc$ and $a= b \cdot c$ for
  some $c \in \mathbbm{N}$.  Now set
  $$
  \begin{array}{rcl}
    T &=& \mn{ind}(\Amc) \\[1mm]
    L_1(x) &=& \{ C \in \mn{cl}(\Tmc_1) \mid x \in C^{\Imc_1} \}
    \\[1mm]
    L_2(x) &=& \{ C \in \mn{CN}(\Tmc_2) \mid \Amc,\Tmc_2 \models C(x)
               \} \\[1mm]
    L_3(x) &=& \left \{
               \begin{array}{rl}
                 1 & \text{ if } x=a_0 \\
                 0 & \text{ otherwise}
               \end{array}
               \right .
  \end{array}
  $$
  It remains to define $L_4$.  Start with setting $L_4(x)=\emptyset$ for
  all~$x$. If Point~1 above is true, we are done. If Point~2 is true, then
  there is a $\Sigmaquery$-successor set $S=\{ \exists R_0 . A, \forall R_0
  . B_1,\dots,\forall R_0 . B_n\}$ for $L_2(a_0)$ such that the restriction of
  $\Imc_{\Tmc_2,\Amc}$ to the subtree-interpretation rooted at $d_0$ is the
  canonical model $\Imc_{\Tmc,\{A,B_1,\dots,B_n\}}$. Set $L_4(a_0)=S$. We
  continue to modify $L_4$, proceeding in rounds. To keep track of the
  modifications that we have already done, we use a set
  $$\Gamma \subseteq
  \mn{ind}(\Amc) \times (\NR \cap \Sigmaquery) \times
  \Delta^{\Imc_{\Tmc_2,\Amc}}
   $$
   such that the following conditions are satisfied:
   \begin{itemize}

   \item[(i)] if $(a,R,d) \in \Gamma$, then $L_4(a)$ has the form $\{ \exists R
     . A, \forall R . B_1,\dots,\forall R . B_n\}$ and the restriction of
     $\Imc_{\Tmc_2,\Amc}$ to the subtree-interpretation rooted at $d$ is the
     canonical model $\Imc_{\Tmc,\{A,B_1,\dots,B_n\}}$;

   \item[(ii)] if $(a,R,d) \in \Gamma$ and $d'$ is an $R$-successor of
     $a$ in $\Imc_1$, then $(\Imc_{\Tmc_2,\Amc},d)
     \not\leq_{\Sigmaquery} (\Imc_1,d')$.

   % \item[($*$)] if $(a,r,d) \in \Gamma$ and $b$ is an $r$-successor of
   %   $a$ in \Amc, then $(\Imc_{\Tmc_2,\Amc},d)$ is not
   %   {\color{blue}$\Sigma$-simulated by} $(\Imc_1,b)$.

   \end{itemize}
   Initially, set $\Gamma = \{ (a_0,R_0,d_0) \}$.  In each round of
   the modification of $L_4$, iterate over all elements $(a,R,d) \in
   \Gamma$ that have not been processed in previous rounds. Let
   $L_4(a)= \{ \exists R . A, \forall R . B_1,\dots,\forall R . B_n\}$
   and iterate over all $R$-successors $b$ of $a$ in \Amc. By (ii),
   $(\Imc_{\Tmc_2,\Amc},d) \not\leq_{\Sigmaquery} (\Imc_1,b)$. By (i),
   there is thus a top-level $\Sigmaquery$-concept name $A'$ in $A
   \sqcap B_1 \sqcap \cdots \sqcap B_n$ such that $b \notin
   A^{\Imc_1}$ or there is an $R'$-successor $d'$ of $d$ in
   $\Imc_{\Tmc_2,\Amc}$, $R'$ a $\Sigmaquery$-role name, such that for
   all $R'$-successors $d''$ of $b$ in $\Imc_1$,
   $(\Imc_{\Tmc_2,\Amc},d') \not\leq_{\Sigmaquery} (\Imc_1,d'')$. In the
   former case, do nothing. In the latter case, there is a
   $\Sigmaquery$-successor set $S'=\{ \exists R' . A', \forall R'
   . B'_1,\dots,\forall R' . B'_{n'}\}$ for $\{A,B_1,\dots,B_n\}$ such
   that the restriction of $\Imc_{\Tmc_2,\Amc}$ to the
     subtree-interpretation rooted at $d'$ is the canonical model
     $\Imc_{\Tmc,\{A',B'_1,\dots,B'_{n'}\}}$. Set $L_4(b)=S'$ and add $(b,R',d')$ to
   $\Gamma$.

   Since we are following only role names (but not inverse roles)
   during the modification of $L_4$ and since \Amc is tree-shaped, we
   will never process tuples $(a_1,R_1,d_1), (a_2,R_2,d_2)$ from
   $\Gamma$ such that $a_1=a_2$. For any $x$, we might thus only
   redefine $L_4(x)$ from the empty set to a non-empty set, but never
   from one non-empty set to another. For the same reason, the
   definition of $L_4$ finishes after finitely many rounds.

   It can be verified that the $\Gamma$-labeled tree $(T,L)$ just
   constructed is $i$-proper for all $i \in \{0,\dots,4\}$. The
   most interesting point is 4-properness, which consists of four
   conditions. Condition~1 is satisfied by construction of $L_4$.
   Condition~2 is satisfied by ($*$) and Conditions~3 and~4 again
   by construction of $L_4$.
\end{proof}

\subsection{Upper Bound in Theorem~\ref{thm:exptbox}}
\label{subsect:autofull}

By Theorem~\ref{thm:first} and Lemma~\ref{lem:gammattrees}, we can
decide whether $\Tmc_1$ does $(\Sigma_1,\Sigma_2)$-rCQ entail $\Tmc_2$
by checking that there is no $\Gamma$-labeled tree that is $i$-proper
for each $i \in \{0,\dots,4\}$. We do this by constructing automata
$\Amc_0,\dots,\Amc_4$ such that each $\Amc_i$ accepts exactly the
$\Gamma$-labeled trees that are $i$-proper, then intersecting the
automata and finally testing for emptiness. Some of the
constructed automata are \TWABAs while others are NTAs. Before intersecting,
all \TWABAs are converted into equivalent NTAs (which involves an
exponential blowup). Emptiness of NTAs can be decided in time
polynomial in the number of states. To achieve \ExpTime overall
complexity, the constructed \TWABAs should thus have at most
polynomially many states while the NTAs can have at most (single)
exponentially many states.% \footnote{\color{blue}This is all a bit
  % sloppy; but do we really want to give full details on the sizes of
  % transition relations etc? just looks messy, but is not very
  % insightful...}
It is straightforward to construct
\begin{enumerate}

\item an NTA $\Amf_0$ that checks 0-properness and has constantly many
  states;

\item a \TWABA $\Amf_1$ that checks 1-properness and whose number of
  states is polynomial in $|\Tmc_1|$ (note that Conditions~1 and~2 of
  1-properness are in a sense trivial as they could also be guaranteed
  by removing undesired symbols from the alphabet $\Gamma$);

\item an NTA $\Amf_3$ that checks 3-properness and has constantly many
  states;

\item an NTA $\Amf_4$ that checks 4-properness and whose number of
states is (single) exponential in $|\Tmc_2|$ (note that Conditions~1
and~2 of 4-properness could again be ensured by refining $\Gamma$).

\end{enumerate}
Details are omitted. It thus remains to construct an automaton
$\Amf_2$ that checks 2-properness.  For this purpose, it is more
convenient to use a \TWABA than an NTA. In fact, the reason for mixing
\TWABAs and NTAs is that while $\Amf_2$ is more easy to be constructed
as a \TWABA, there is no obvious way to construct $\Amf_4$ as a \TWABA
with only polynomially many states: it seems one needs that one state
is needed for every possible value of the $L_4$-components in
$\Gamma$-labels.

The \TWABA $\Amf_2$ is actually the intersection of two \TWABAs
$\Amf_{2,1}$ and $\Amf_{2,2}$. The \TWABA $\Amf_{2,1}$ ensures one
direction of Condition~1 of 2-properness as well as Condition~2,
that is:
\begin{itemize}

\item[(i)] if $\Amc_{(T,L)}$ is consistent w.r.t.\ $\Tmc_2$, then
  $\Amc_{(T,L)},\Tmc_2 \models A(x)$ implies $A \in L_2(x)$ for all $x
  \in T$ and $A \in \mn{CN}(\Tmc_2)$;

\item[(ii)] if $A \in L_2(x)$, then $A \sqsubseteq \bot \notin \Tmc_2$.

\end{itemize}
It is simple for a \TWABA to verify (ii), alternatively one could
refine $\Gamma$.  To achieve~(i), it suffices to guarantee the
following conditions for all $x_1,x_2 \in T$, which are essentially
just the rules of a chase required for Horn-\ALC TBoxes in normal
form:
\begin{enumerate}

\item $A \in L_0(x_1)$ implies $A \in L_2(x_1)$;

\item if $A_1,\dots,A_n \in L_2(x_1)$ and $\Tmc_2 \models A_1
  \sqcap \cdots \sqcap A_n \sqsubseteq A$, then $A \in L_2(x_1)$;

\item if $A \in L_2(x_1)$, $x_2$ is a successor of $x_1$,
  $R \in L_0(x_2)$, and $A \sqsubseteq \forall R . B \in \Tmc_2$,
  then $B \in L_2(x_2)$;

\item if $A \in L_2(x_2)$, $x_2$ is a successor of $x_1$,
  $R^- \in L_0(x_2)$, and $A \sqsubseteq \forall R . B \in \Tmc_2$,
  then $B \in L_2(x_1)$;

\item if $A \in L_2(x_2)$, $x_2$ is a successor of $x_1$,
  $R \in L_0(x_2)$, and $\exists R . A \sqsubseteq B \in \Tmc_2$,
  then $B \in L_2(x_1)$;

\item if $A \in L_2(x_1)$, $x_2$ is a successor of $x_1$,
  $R^- \in L_0(x_2)$, and $\exists R . A \sqsubseteq B \in \Tmc_2$,
  then $B \in L_2(x_2)$

\end{enumerate}
All of this is easily verified with a \TWABA, details are again
ommitted. Note that Conditions~1 and~2 can again be ensured by
refining $\Gamma$.

The purpose of $\Amf_{2,2}$ is to ensure the converse of (i). Before
constructing it, it is convenient to first characterize the entailment
of concept names at ABox individuals in terms of derivation trees.
%  and let $\Tmc_\exists$ be the restriction of
% $\Tmc_2$ to CIs of the form $\exists r . A \sqsubseteq B$, with $r$ a
% (potentially inverse) role.  {\color{red}???}
A \emph{$\Tmc_2$-derivation tree} for an assertion $A_0(a_0)$ in \Amc
with $A_0 \in \mn{CN}(\Tmc_2)$ is a finite $\mn{ind}(\Amc) \times
\mn{CN}(\Tmc_2)$-labeled tree $(T,V)$ that satisfies
the following conditions:
\begin{itemize}

\item $V(\varepsilon)=(a_0,A_0)$;

%\item if %$x \neq \varepsilon$ and
%$V(x)=(a,\bot)$, then $x=\varepsilon$;

% \item if $V(x)=(a,A)$ and $A(a) \in \Amc$ or $\top \sqsubseteq A \in
%   \Tmc$, then $x$ is a leaf;

% \item if $V(x)=(a,A)$, then $x$ has one successor $y$ with $V(y)=(a,\Gamma)$
%   for some $\Gamma$ with $\Tmc \models \Gamma \sqsubseteq A$;

\item if $V(x)=(a,A)$ and neither $A(a) \in \Amc$ nor \mbox{$\top
  \sqsubseteq A \in \Tmc_2$}, then one of the following holds:
  \begin{itemize}

  \item $x$ has successors $y_1,\dots,y_n$ with
    $V(y_i)=(a,A_i)$ for $1 \leq i \leq n$ and $\Tmc_2 \models A_1
    \sqcap \cdots \sqcap A_n \sqsubseteq A$;
    % (then $x$ is of  \emph{local type});

  \item $x$ has a single successor $y$ with $V(y)=(b,B)$ and there is
    an $\exists R . B \sqsubseteq A \in \Tmc_2$ such that
    $R(a,b) \in \Amc$;
    % (then $x$ is of \emph{existential type}).

  \item $x$ has a single successor $y$ with $V(y)=(b,B)$ and
    there is a $B \sqsubseteq \forall R . A \in \Tmc_2$ such
    that $R(b,a) \in \Amc$.

  \end{itemize}

\end{itemize}
%
% Note that there might be more than one derivation tree for the same
% assertion $A_0(a_0)$. Also note that derivations trees are essentially
% the same thing as proof trees for datalog.
%We call a TBox \Tmc \emph{satisfiable} if it has a model.
%The main property of derivation trees is the following.
%
\begin{lemma}
\label{lem:derivationtrees}
%~\\[-4mm]
  %
  %\begin{enumerate}
  %
  % \item $\Amc,\Tmc_2 \models A(a)$ iff \Amc is inconsistent w.r.t.\
  %   $\Tmc_2$ or there is a derivation tree for $A(a)$ in \Amc, for all
  %   assertions $A(a)$ with $A \in \NC$ and $a \in \mn{ind}(\Amc)$;
  %
  % \item \Amc is inconsistent w.r.t.\ $\Tmc_2$ iff $\Tmc_2$ is
  %   unsatisfiable or there is a derivation tree for $\bot(a)$ in \Amc,
  %   for some $a \in \mn{ind}(\Amc)$.
  %
  %\item
If $\Amc,\Tmc_2 \models A(a)$ and \Amc is consistent w.r.t.\
    $\Tmc_2$, then there is a derivation tree for $A(a)$ in \Amc, for
    all assertions $A(a)$ with $A \in \mn{CN}(\Tmc_2)$ and $a \in \mn{ind}(\Amc)$.
%
  % \item \Amc is inconsistent w.r.t.\ $\Tmc_2$ iff $\Tmc_2$ is
  %   unsatisfiable or  there is a derivation tree for $\bot(a)$ in \Amc,
  %   for some $a \in \mn{ind}(\Amc)$.
  %
  %
  % \end{enumerate}
\end{lemma}
A proof of Lemma~\ref{lem:derivationtrees} is based on the chase
procedure, details can be found in \cite{BienvenuLW-ijcai-13}
for the extension $\mathcal{ELI}_\bot$ of Horn-\ALC.

We are now ready to construct the remaining \TWABA~$\Amf_{2,2}$.  By
Lemma~\ref{lem:derivationtrees} and since $\Amf_{2,1}$ ensures
that $\Amc_{(T,L)}$ is consistent w.r.t.\ $\Tmc_2$, it is enough for
$\Amf_{2,2}$ to verify that, for each node $x \in T$ and each concept
name $A \in L_2(x)$, there is a $\Tmc_2$-derivation tree for $A(x)$ in
$\Amc_{(T,L)}$.

For readability, we use $\Gamma^- := \Gamma_0 \times \mn{CN}(\Tmc_2)$ as
the alphabet instead of $\Gamma$ since transitions of $\Amf_{2,2}$
only depend on the $L_0$- and $L_2$-components of $\Gamma$-labels. Let
$\mn{rol}(\Tmc_2)$ be the set of all roles $R,R^-$ such that the role
name $R$ occurs in $\Tmc_2$.  Set $\Amf_2=(Q,\Gamma^-,\delta,q_0,R)$
with
  $$
  \begin{array}{rcl}
  Q &=& \{
  q_0 \} \uplus \{ q_A \mid A \in \mn{CN}(\Tmc_2) \} %\cup \{ \bot \} \}
   \uplus \{ q_{A,R}, q_R \mid A \in \mn{CN}(\Tmc_2), %\cup \{ \bot \},
     R \in \mn{rol}(\Tmc_2) \}
  \end{array}
  $$
  and $R = \emptyset$ (i.e., exactly the finite runs are
  accepting).
% For all $(\sigma_0,\sigma_2) \in \Gamma^-$ such that $C \in \sigma_2$
%   and $D \notin \sigma_2$ for some $C \sqsubseteq D \in \Tmc_2$, set
%   %
%   $$
%     \delta(q_0,(\sigma_0,\sigma_2)) = \bot.
%   $$
  %
  For all $(\sigma_0,\sigma_2) \in \Gamma^-$, set
  \begin{itemize}

  \item  $\delta(q_0,(\sigma_0,\sigma_2)) = \displaystyle \bigwedge_{A
      \in \sigma_2} (0,q_A) \wedge (\mn{leaf} \vee \bigwedge_{i \in 1..m} (i,q_0))$;
%{\color{red}stop at leaves}

\item $\delta(q_A,(\sigma_0,\sigma_2))=\mn{true}$ whenever $A \in \sigma_1$ or $\top
  \sqsubseteq A \in \Tmc_2$;

\item $\delta(q_A,(\sigma_0,\sigma_2))=
  \begin{array}[t]{@{}l}
    % \!\!\!\!\!\!\!\!
    \bigvee_{\Tmc_2 \models A_1 \sqcap \cdots \sqcap A_n \sqsubseteq A}
    %\!\!\!\!\!\!\!\!
    ((0,q_{A_1}) \wedge \cdots \wedge (0,q_{A_n})) \vee{}\\
    \bigvee_{\exists R . B \sqsubseteq A \in \Tmc, \ R \in \Sigmaabox}
    (((0,q_{R^-}) \wedge (-1,q_{B})) \vee
    \bigvee_{i \in 1..m} (i,q_{B,R})) \vee{}\\
    \bigvee_{B \sqsubseteq \forall R . A \in \Tmc, \ R \in \Sigmaabox}
    ((0,q_{R}) \wedge (-1,q_{B})) \vee \bigvee_{i \in 1..m} (i,q_{B,{R^-}}))
  \end{array}$ \\[2mm]
  whenever $A \notin \sigma_0$ and $\top \sqsubseteq A \notin \Tmc_2$;

\item $\delta(q_{A,R},(\sigma_0,\sigma_2))= (0,q_A)$ whenever $R \in \sigma_0$;

\item $\delta(q_{A,R},(\sigma_0,\sigma_2))= \mn{false}$ whenever $R \notin \sigma_0$;

\item $\delta(q_{R},(\sigma_0,\sigma_2))= \mn{true}$ whenever $R \in \sigma_0$;

\item $\delta(q_{R},(\sigma_0,\sigma_2))= \mn{false}$ whenever $R \notin \sigma_0$.

  \end{itemize}
  Note that the finiteness of runs ensures that $\Tmc_2$-derivation
  trees are also finite, as required.
%
%   The remaining automaton $\Amf_{2,3}$ has to ensure that
%   $\Amc_{(T,L)}$ is consistent w.r.t.\ $\Tmc_2$. As already mentioned,
%   it is rather similar to $\Amf_{2,2}$ and we only sketch the
%   differences. We add a state $q_\bot$ and replace the initial
%   transition with
%   %
%   $$
%   \delta(q_0,(\sigma_0,\sigma_2)) = \displaystyle q_\bot \vee \bigvee_{i \in 1..m} (i,q_0).
%   $$
% {\color{red}stop at leaves}
%   %
% The resulting automaton ensures that there is some node $x \in T$ such
% that there is a $\Tmc_2$-derivation tree of $\bot(a)$ in
% $\Amc_{(T,L)}$. As $\Amf_{2,3}$, we use its complementation.
% Note that we can assume w.l.o.g.\ that $\Tmc_2$ is satisfiable
% since this can be checked in \ExpTime and, otherwise, $\Tmc_1$
% trivially $(\Sigma_1,\Sigma_2)$-entails $\Tmc_2$. Consequently,
% by Point~2 of Lemma~\ref{lem:derivationtrees} the automaton
% $\Amf_{2,3}$ verified consistency of $\Amc_{(T,L)}$ with $\Tmc_2$,
% as desired.

\subsection{Upper Bound in Theorem~\ref{thm:2exptbox}}

The 2\ExpTime upper bound stated in Theorem~\ref{thm:2exptbox} can be
obtained by a modification of the construction given in
Section~\ref{subsect:autofull}. We now have to build in the
characterization given in Theorem~\ref{thm:first} instead of the one
from Theorem~\ref{thm:second}. There are two differences: first, the
theorem refers to the canonical model $\Imc_{\Tmc_1,\Amc}$ instead of
quantifying over all models \Imc of $(\Tmc_1,\Amc)$; and second, we
need to consider $\Sigma_2$-homomorphic embeddability instead of
con-$\Sigma_2$-homomorphic embeddability. The former difference can be
ignored. In fact, Theorem~\ref{thm:second} remains true if we quantify
over all models \Imc of $(\Tmc_1,\Amc)$, as in
Theorem~\ref{thm:first}, because $\Imc_{\Tmc_1,\Amc}$ is
$\Sigma_2$-homomorphically embeddable into any model of $\Tmc_1$ and
\Amc. The second difference, however, does make a difference. To
understand it more properly, we first give the following adaptation of
Lemma~\ref{lem:homtosim}.
\begin{lemma}
\label{lem:homtosim2}
Let \Amc be a $\Sigmaabox$-ABox and $\Imc_1$ a model of
$(\Tmc_1,\Amc)$. Then $\Imc_{\Tmc_2,\Amc}$ is not $\Sigmaquery$-homomorphically
embeddable into $\Imc_1$ iff there is an $a \in \mn{ind}(\Amc)$ such
that one of the following is true:
  \begin{enumerate}

  \item there is a $\Sigmaquery$-concept name $A$ with
    $a \in A^{\Imc_{\Tmc_2,\Amc}} \setminus A^{\Imc_1}$;

  \item there is an $R_0$-successor $d_0$ of $a$ in
    $\Imc_{\Tmc_2,\Amc}$, for some $\Sigmaquery$-role name $R_0$, such
    that $d_0 \notin \mn{ind}(\Amc)$ and for all $R_0$-successors $d$
    of $a$ in $\Imc_1$, we have that $(\Imc_{\Tmc_2,\Amc},d_0)
    \not\leq_{\Sigmaquery}(\Imc_1,d)$.

  \item there is an element $d$ in the subtree of
      $\Imc_{\Tmc_2,\Amc}$ rooted at $a$ (with possibly $d=a$) and $d$ has an
    $R_0$-successor $d_0$, for some role name $R_0 \notin
    \Sigmaquery$, such that for all elements $e$ of $\Imc_1$, we have
    $(\Imc_{\Tmc_2,\Amc},d_0) \not\leq_{\Sigmaquery}(\Imc_1,e)$.

  \end{enumerate}
\end{lemma}
The proof of Lemma~\ref{lem:homtosim2} is very similar to that of
Lemma~\ref{lem:homtosim}, details are omitted.  Note that the
difference between Lemma~\ref{lem:homtosim} and
Lemma~\ref{lem:homtosim2} is the additional Condition~3 in the
latter. This condition needs to be reflected in the definition of
proper $\Gamma$-labeled trees which, in turn, requires a
modification of the alphabet~$\Gamma$.

An important reason for the construction in
Section~\ref{subsect:autofull} to yield an \ExpTime upper bound is
that in the $L_4$-component of $\Gamma$-labels, we only need to store
a single successor set instead of a set of such sets. This is not the
case in the new construction (which only yields 2\ExpTime upper bound)
where we let the $L_4$-component of $\Gamma$-labels range over
$2^{2^{\mn{sub}(\Tmc_2)}}$ instead of over $2^{\mn{sub}(\Tmc_2)}$. We
also add an $L_5$-component to $\Gamma$-labels, which also ranges over
$2^{2^{\mn{sub}(\Tmc_2)}}$. The notion of $i$-properness remains the
same for $i \in \{0,1,2,3\}$. We adapt the notion of 4-properness and
add a notion of 5-properness.

As a preliminary, we need to define the notion of a descendant set.
Let $t \subseteq \mn{CN}(\Tmc_2)$ and define $\Gamma$ to be the
smallest set such that
\begin{itemize}

\item $t \in \Gamma$;

\item if $t' \in \Gamma$, $A \in t'$, and $A' \sqsubseteq \exists R . A
  \in \Tmc_2$, then $\{ A,B_1,\dots,B_n\} \in \Gamma$ where
  $B_1,\dots,B_n$ is the set of all concept names such that, for some
  $B \in t'$, we have $B \sqsubseteq \forall R . B_i \in \Tmc_2$.

\end{itemize}
Note that, in the above definition, $R$ need not be from $\Sigmaquery$
(nor from its complement). A subset $s$ of $\mn{CN}(\Tmc_2)$ is a
\emph{descendant set} for $t$ if there is a $t' \in \Gamma$, an $A \in
t'$, and an $A' \sqsubseteq \exists R . A \in \Tmc_2$ with $R \notin
\Sigmaquery$ such that $s$ consists of $A$ and of all concept names
$B$ such that $B' \sqsubseteq \forall R . B \in \Tmc_2$ for some $B'
\in t'$.

A $\Gamma$-labeled tree $(T,L)$ is \emph{4-proper} if it satisfies
the following conditions for all $x_1,x_2 \in T$:
\begin{enumerate}

\item if $L_3(x_1)=1$, then one of the following is true:
  \begin{itemize}
  \item
  there is a $\Sigmaquery$-concept name in $L_2(x_1)
  \setminus L_1(x_1)$;

  \item or $L_4(x_1)$ contains
% a set
%   %
%   $$
%     \{ \exists r . C, \forall r . D_1, \cdots \forall r . D_n \}
%   $$
%   %
%   such that {\color{blue} $\Tmc \models L_2(x) \sqsubseteq \exists u . \midsqcap
%   L_4(x)$;}
  a $\Sigma_2$-successor set for~$L_2(x_1)$;

\item $L_5(y)$ contains a $\Sigma_2$-descendant set for~$L_2(x_1)$;

  \end{itemize}

\item there is a model \Imc of $\Tmc_1$ and a $d \in \Delta^\Imc$ such
  that all of the following are true:
  \begin{itemize}

  \item $d \in C^\Imc$ iff $C \in L_1(x_1)$ for all $C \in
    \mn{cl}(\Tmc_1)$;

  \item if $S \in L_4(x_1)$, then
    $(\Imc_{\Tmc_2,S},a_\varepsilon) \not\leq_{\Sigmaquery} (\Imc,d)$;

  \item if $S \in L_5(x_1)$ and $e \in \Delta^\Imc$, then
    $(\Imc_{\Tmc_2,S},a_\varepsilon)
    \not\leq_{\Sigmaquery} (\Imc,e)$;

  \end{itemize}

% \item if $L_3(x) \neq \emptyset$, then for all successor sets $S$ from
%   $L_1(x)$, there is {\color{blue}no $\Sigma$-simulation from
%     $\Imc_{\Tmc_2,L_3(x)}$ to
%     $\Imc_{\Tmc_1,S}$;\footnote{\color{blue}here and elsewhere: fix
%       notation}} {\color{red}CANONICAL!!!}

\item if $x_2$ is a child of $x_1$, $L_0(x_2)$ contains the role name
  $R$, and $L_4(x_1) \ni \{ \exists R . A, \forall R . B_1, \dots,\forall
  R . B_n \}$, then
  %
%  \begin{enumerate}
%  \item
there is a $\Sigmaquery$-concept name in
  $\mn{cl}_{\Tmc_2}(\{A,B_1,\dots,B_n\}) \setminus L_1(x_2)$ or
%  \item
$L_4(x_2)$ contains
  a $\Sigmaquery$-successor set for $\mn{cl}_{\Tmc_2}(\{A,B_1,\dots,B_n\})$;
%  \end{enumerate}

\item if $x_2$ is a child of $x_1$, $L_0(x_2)$ contains the role
  $R^-$, and $L_4(x_2) \ni \{ \exists R . A, \forall R . B_1,
  \dots,\forall R . B_n \}$, then
  %
%  \begin{enumerate}
%
%  \item
there is a $\Sigmaquery$-concept name in
  $\mn{cl}_{\Tmc_2}(\{A,B_1,\dots,B_n\}) \setminus L_1(x_1)$ or
%
 % \item
$L_4(x_1)$ contains
  a $\Sigmaquery$-successor set for $\mn{cl}_{\Tmc_2}(\{A,B_1,\dots,B_n\})$.
%  \end{enumerate}
%

% \item if $L_4(x_1)=\{ \exists r . A, \forall r . B_1,\dots, \forall r
%   . B_n \}$, then $x_1$ has an $r$-successor in $\Amc_{(T,L)}$.

\end{enumerate}
A $\Gamma$-labeled tree $(T,L)$ is \emph{5-proper} if all $x \in T$
agree regarding their $L_5$-label.

Note how the adapted notion of 4-properness and the $L_5$-component of
$\Gamma$-labels implements the additional third condition of
Lemma~\ref{lem:homtosim2}. That condition gives rise to an additional
set of simulations that have to be avoided. The (pointed)
interpretations on the ``source side'' of these simulations are
described using sets of concepts in $L_5$. In the pointed
interpretations $(\Imc_1,e)$ on the ``target side'', we now have to
consider all possible points $e$. For this reason, 5-properness
distributes elements of $L_5$-labels to everywhere else. The
simulations are then avoided via the additional third item in the
second condition of 4-properness. The proof details of the following
lemma are omitted.
\begin{lemma}
\label{lem:gammattrees}
  % $\Tmc_1$ does not $\Sigmaquery$-CQ entail $\Tmc_2$ iff there is an
  % $m$-ary $\Gamma$-labeled tree that is $i$-proper for all $i \in
  % \{0,\dots,4\}$.
There is an $m$-ary $\Gamma$-labeled tree that is $i$-proper for all
$i \in \{0,\dots,5\}$ iff there is a tree-shaped $\Sigmaabox$-ABox
$\Amc$ of outdegree at most $m$ that is consistent w.r.t.\ $\Tmc_1$
and $\Tmc_2$ and a model $\Imc_1$ of
$(\Tmc_1,\Amc)$ such that the canonical model $\Imc_{\Tmc_2,\Amc}$ of
$(\Tmc_2,\Amc)$ is not $\Sigmaquery$-homomorphically embeddable
into $\Imc_1$.
\end{lemma}
It is now straightforward to adapt the automaton construction to the
new version of 4-properness, and to add an automaton for 5-properness.
The NTA for 4-properness will now have double exponentially many
states because $L_4$- and $L_5$-components are sets of sets of
concepts instead of sets of concepts. In fact, we could dispense NTAs
altogether and use an \TWABA that has exponentially many
states. Overall, we obtain a 2\ExpTime upper bound.

\subsection{2\ExpTime Lower Bound}

We reduce the word problem of
exponentially space bounded alternating Turing machines (ATMs), see
\cite{ChandraKS81}.  An \emph{Alternating Turing Machine (ATM)}
is of the form $M = (Q,\Sigma,\Gamma,q_0,\Delta)$. The set
of \emph{states} $Q = Q_\exists \uplus Q_\forall \uplus \{q_a\} \uplus
\{q_r\}$ consists of \emph{existential states} in $Q_\exists$,
\emph{universal states} in $Q_\forall$, an \emph{accepting state}
$q_a$, and a \emph{rejecting state} $q_r$; $\Sigma$ is the \emph{input
  alphabet} and $\Gamma$ the \emph{work alphabet} containing a
\emph{blank symbol} $\square$ and satisfying $\Sigma \subseteq
\Gamma$; $q_0 \in Q_\exists \cup Q_\forall$ is the \emph{starting}
state; and the \emph{transition relation} $\Delta$ is of the form
$$
  \Delta \; \subseteq \; Q \times \Gamma \times Q \times \Gamma
  \times \{ L,R \}.
$$
We write $\Delta(q,\sigma)$ to denote $\{ (q',\sigma',M) \mid
(q,\sigma,q',\sigma',M) \in \Delta \}$ and assume w.l.o.g.\ that every
set $\Delta(q,\sigma)$ contains exactly two elements when $q$ is
universal, and that the state $q_0$ is existential and cannot be
reached by any transition.
%$\Delta(q_r,a) = \emptyset$ for all $a \in \Gamma$.

A \emph{configuration} of an ATM is a word $wqw'$ with $w,w' \in
\Gamma^*$ and $q \in Q$. The intended meaning is that the one-side
infinite tape contains the word $ww'$ with only blanks behind it, the
machine is in state $q$, and the head is on the symbol just after
$w$. The \emph{successor configurations} of a configuration $wqw'$ are
defined in the usual way in terms of the transition
relation~$\Delta$. A \emph{halting configuration} (resp.\
\emph{accepting configuration}) is of the form $wqw'$ with $q \in \{
q_a, q_r \}$ (resp.\ $q=q_a$).

A \emph{computation tree} of an ATM $M$ on input $w$ is a tree whose
nodes are labeled with configurations of $M$ on $w$, such that the
descendants of any non-leaf labeled by a universal (resp.\
existential) configuration include all (resp. one) of the successors
of that configuration. A computation tree is \emph{accepting} if the
root is labeled with the \emph{initial configuration} $q_0w$ for $w$
and all leaves with accepting configurations. An ATM $M$ accepts
input $w$ if there is a computation tree of $M$ on $w$.

% A \emph{computation} of an ATM $M$ on a word $w$ is a
% (finite or infinite) sequence of configurations $K_0,K_1,\dots$ such
% that $K_0=q_0w$ and $K_{i+1}$ is a successor configuration of $K_i$
% for all $i \geq 0$.  The ATMs considered in the following have only
% \emph{finite} computations on any input. Since this case is simpler
% than the general one, we define acceptance for ATMs with finite
% computations, only.
% %, and refer to \cite{Chandra-et-al-81} for the full
% %definition.
% Let $M$ be such an ATM. A halting configuration is
% \emph{accepting} iff it is of the form $wq_aw'$.  For other
% configurations $K=w q w'$, acceptance depends on $q$: if $q \in
% Q_\exists$, then $K$ is accepting iff at least one successor
% configuration is accepting; if $q \in Q_\forall$, then $K$ is
% accepting iff all successor configurations are accepting.  Finally,
% the ATM $M$ with starting state $q_0$ \emph{accepts} the
% input $w$ iff the \emph{initial configuration} $q_0w$ is accepting.
% We use $L(M)$ to denote the language accepted by
% $M$.

\smallskip

There is an exponentially space bounded ATM $M$ whose word
problem is {\sc 2Exp\-Time}-hard and we may assume that the length of
every computation path of $M$ on $w \in \Sigma^n$ is bounded
by $2^{2^{n}}$, and all the configurations $wqw'$ in such computation
paths satisfy $|ww'| \leq 2^{n}$, see \cite{ChandraKS81}. % We may
% also assume w.l.o.g.\ that $M$ never attempts to move left
% on the left-most tape cell.
We may also assume w.l.o.g.\ that $M$ makes at least one step on every
input, and that it never reaches the last tape cell (which is both not
essential for the reduction, but simplifies it).

\medskip Let $w$ be an input to $M$.  We aim to construct Horn-\ALC
TBoxes $\Tmc_1$ and $\Tmc_2$ and a signature $\Sigma$ such that
the following are equivalent:
\begin{enumerate}

\item there is a tree-shaped $\Sigma$-ABox \Amc\xspace
such that
  \begin{enumerate}
  \item \Amc is consistent w.r.t.\ $\Tmc_1$ and $\Tmc_2$ and

  \item $\Imc_{\Tmc_2,\Amc}$ is
    not $\Sigma$-homomorphically embeddable into
    $\Imc_{\Tmc_1,\Amc}$;

  \end{enumerate}

\item $M$ accepts $w$.

\end{enumerate}
Note that we dropped the outdegree condition from
Theorem~\ref{thm:second}. In fact, it is easy to go through the
proofs of that theorem and verify that this condition is not needed;
we have included it because it makes the upper bounds easier.

When dealing with an input $w$ of length $n$, we represent
configurations of $M$ by a sequence of $2^n$ elements linked by the
role name $R$, from now on called \emph{configuration
  sequences}. These sequences are then interconnected to form a
representation of the computation tree of $M$ on $w$. This is
illustrated in Figure~\ref{fig:red3}, which shows three configuration
sequences, enclosed by dashed boxes. The topmost configuration is
universal, and it has two successor configurations. All solid arrows
denote $R$-edges. We will explain later why successor configurations
are separated by two consecutive edges instead of by a single one.
\begin{figure}[tb]
  \centering
    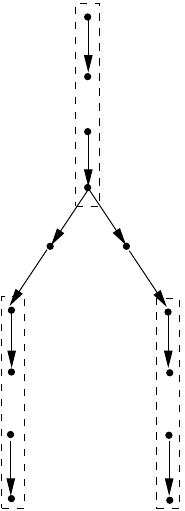
    \caption{Configuration tree (partial)}
    \label{fig:red3}
\end{figure}

The above description is actually an oversimplification. In fact,
every configuration sequence stores two configurations instead of only
one: the current configuration and the previous configuration in the
computation. We will later use the homomorphism condition~(a) above to
ensure that
\begin{itemize}

\item[($*$)] the previous configuration stored in a configuration
sequence is identical to the current configuration stored in its
predecessor configuration sequence.

\end{itemize}
The actual transitions of $M$ are
then represented locally inside configuration sequences.

We next show how to use the TBox $\Tmc_2$ to verify the existence of
a computation tree of $M$ on input $w$ in the ABox,
assuming ($*$).  The signature $\Sigma$ consists of the following
symbols:
\begin{enumerate}

\item concept names $A_0,\dots,A_{n-1}$ and
  $\overline{A}_0,\dots,\overline{A}_{n-1}$ that serve as bits in the
  binary representation of a number between 0 and $2^{n}-1$,
  identifying the position of tape cells inside configuration
  sequences ($A_0$, $\overline{A}_0$ represent the lowest bit);

\item the concept names $A_\sigma$, $A'_\sigma$, $\overline{A}_\sigma$
  for each $\sigma \in \Gamma$;

\item the concept names $A_{q,\sigma}$, $A'_{q,\sigma}$, $\overline{A}_{q,\sigma}$ for
  each $\sigma \in \Gamma$ and $q \in Q$;

% \item the concept names $\overline{H}$, $W$, and $\overline{W}$
%  which stand for ``cell without head'', ``cell being written to reach
% current configuration'', and ``cell not being written to reach current
% configuration'';

% \item concept names $C$ and $P$ which stand for ``current''
%    and ``previous'';

% \item the concept name $A_{q,\sigma,M}$ for each $q \in Q$, $\sigma \in
%    \Gamma$, and $M \in \{L,R\}$ to describe transitions of $M$;

%\item a concept name $I$ that marks the initial configuration;

\item concept names $X_L,X_R$ that mark left and right successor
  configurations;

\item the role name $R$.

\end{enumerate}
From the above list, concept names $A_\sigma$ and $A_{q,\sigma}$ are
used to represent the current configuration and $A'_\sigma$ and
$A'_{q,\sigma}$ for the previous configuration. The role of the
concept names $\overline{A}_\sigma$ and $\overline{A}_{q,\sigma}$ will
be explained later.

We start with verifying accepting configurations, in a bottom-up manner:
$$
\begin{array}{@{}r@{\,}c@{\,}l}
  A_0 \sqcap \cdots \sqcap A_{n-1} \sqcap A_\sigma \sqcap A'_{\sigma}
  &\sqsubseteq& V \\[1mm]
  % A_0 \sqcap \cdots \sqcap A_{n-1} \sqcap A_\sigma \sqcap A'_{q,\sigma'}
  % &\sqsubseteq& V_{L,\sigma} \\[1mm]
  % A_0 \sqcap \cdots \sqcap A_{n-1} \sqcap A_{q_\mn{acc},\sigma} \sqcap A'_\alpha
  % &\sqsubseteq& V_{R,q_{\mn{acc}}} \\[1mm]
  A_i \sqcap \exists R . A_i \sqcap \midsqcup_{j < i} \exists R
  . A_j &\sqsubseteq& \mn{ok}_i  \\[1mm]
  \overline{A}_i \sqcap \exists R . \overline{A}_i \sqcap \midsqcup_{j < i} \exists R
  . A_j &\sqsubseteq& \mn{ok}_i  \\[1mm]
  A_i \sqcap \exists R . \overline{A}_i \sqcap \midsqcap_{j < i} \exists R
  . \overline{A}_j &\sqsubseteq& \mn{ok}_i  \\[1mm]
  \overline{A}_i \sqcap \exists R . A_i \sqcap \midsqcap_{j < i} \exists R
  . \overline{A}_j &\sqsubseteq& \mn{ok}_i  \\[1mm]
  \mn{ok}_0 \sqcap  \cdots \sqcap \mn{ok}_{n-1} \sqcap \overline{A}_i \sqcap \exists R . V
  \sqcap A_\sigma \sqcap A'_{\sigma} &\sqsubseteq& V \\[1mm]
  \mn{ok}_0 \sqcap  \cdots \sqcap \mn{ok}_{n-1} \sqcap \overline{A}_i \sqcap \exists R . V
  \sqcap A_\sigma \sqcap A'_{q,\sigma'} &\sqsubseteq& V_{L,\sigma} \\[1mm]
  \mn{ok}_0 \sqcap  \cdots \sqcap \mn{ok}_{n-1} \sqcap \overline{A}_i \sqcap \exists R . V
  \sqcap A_{q_{\mn{acc}},\sigma} \sqcap A'_{\sigma} &\sqsubseteq& V_{R,q_\mn{acc}} \\[1mm]
  \mn{ok}_0 \sqcap  \cdots \sqcap \mn{ok}_{n-1} \sqcap \overline{A}_i \sqcap \exists R . V_{L,\sigma}
  \sqcap A_{q_{\mn{acc}},\sigma'} \sqcap A'_{\sigma'} &\sqsubseteq& V_{L,q_\mn{acc},\sigma} \\[1mm]
  \mn{ok}_0 \sqcap  \cdots \sqcap \mn{ok}_{n-1} \sqcap \overline{A}_i \sqcap \exists R . V_{R,q_{\mn{acc}}}
  \sqcap A_{\sigma} \sqcap A'_{q,\sigma'} &\sqsubseteq& V_{R,q_\mn{acc},\sigma} \\[1mm]
  \mn{ok}_0 \sqcap  \cdots \sqcap \mn{ok}_{n-1} \sqcap \overline{A}_i \sqcap \exists R . V_{M,q_{\mn{acc}},\sigma}
  \sqcap A_{\sigma'} \sqcap A'_{\sigma'} &\sqsubseteq& V_{M,q_\mn{acc},\sigma} \\[1mm]
  \exists R . A_i \sqcap \exists R . \overline{A}_i &\sqsubseteq& \bot
\end{array}
$$
where $\sigma,\sigma'$ range over $\Gamma$, $q$ over $Q$, and
$i$ over $0..n-1$.  The first line starts the verification at the last
tape cell, ensuring that at least one concept name $A_\alpha$ and one
concept name $A'_\beta$ is true. The following lines implement the
verification of the remaining tape cells of the configuration. Lines
two to five implement decrementation of a binary counter and the
conjunct $\overline{A}_i$ in Lines six to eleven prevents the counter
from wrapping around once it has reached zero. We use several kinds
of verification markers:
\begin{itemize}

\item with $V$, we indicate that we have not yet seen the head of the
  TM;

\item $V_{L,\sigma}$ indicates that the TM made a step to the left to
  reach the current configuration, writing $\sigma$;

\item $V_{R,q}$ indicates that the TM made a step to the right to
  reach the current configuration, switching to state $q$;

\item $V_{M,q,\sigma}$ indicates that the TM moved in direction $M$
to reach the current configuration, switching to state $q$ and writing
$\sigma$.

\end{itemize}
In the remaining reduction, we expect that a marker of the form
$V_{M,q,\sigma}$ has been derived at the first cell of the
configuration.  This makes sure that there is exactly one head in the
current and in the previous configuration, and that the head moved
exactly one step between the previous and the current position. Also
note that the above CIs make sure that the tape content does not
change for cells that were not under the head in the previous
configuration. We exploit that $M$ never moves its head to the
right-most tape cell, simply ignoring this case in the CIs above. Note
that it is not immediately clear that lines two to eleven work as
intended since they can speak about different $R$-successors for
different bits. The last line fixes this problem.

We also ensure that relevant concept names are mutually exclusive:
$$
\begin{array}{rcll}
  A_i \sqcap \overline{A}_i &\sqsubseteq& \bot \\[1mm]
  A_{\sigma_1} \sqcap A_{\sigma_2} &\sqsubseteq& \bot & \text{ if }
  \sigma_1 \neq \sigma_2 \\[1mm]
  A_{\sigma_1} \sqcap A_{q_2,\sigma_2} &\sqsubseteq& \bot \\[1mm]
  A_{q_1,\sigma_1} \sqcap A_{q_2,\sigma_2} &\sqsubseteq& \bot & \text{ if }
  (q_1,\sigma_1) \neq (q_2,\sigma_2)
\end{array}
$$
where the $i$ ranges over $0..n-1$, $\sigma_1,\sigma_2$ over $\Gamma$,
and $q_1,q_2$ over~$Q$. We also add the same concept inclusions for
the primed versions of these concept names.  The next step is to
verify non-halting configurations:
$$
\begin{array}{@{}r@{\,}c@{\,}l}
  \exists R. \exists R . (X_L \sqcap \overline{A}_0 \sqcap \cdots \sqcap
  \overline{A}_{n-1} \sqcap (V_{M,q,\sigma} \sqcup V'_{M,q,\sigma})) &\sqsubseteq& L\mn{ok} \\[1mm]
  \exists R . \exists R . (X_R  \sqcap \overline{A}_0 \sqcap \cdots \sqcap
  \overline{A}_{n-1}\sqcap (V_{M,q,\sigma} \sqcup V'_{M,q,\sigma})) &\sqsubseteq& R\mn{ok} \\[1mm]
  A_0 \sqcap \cdots \sqcap A_{n-1} \sqcap A_\sigma \sqcap A'_{\sigma}
  \sqcap L\mn{ok} \sqcap R\mn{ok}   &\sqsubseteq& V' \\[1mm]
  \mn{ok}_0 \sqcap  \cdots \sqcap \mn{ok}_{n-1} \sqcap \overline{A}_i \sqcap \exists R . V'
  \sqcap A_\sigma \sqcap A'_{\sigma} &\sqsubseteq& V' \\[1mm]
  \mn{ok}_0 \sqcap  \cdots \sqcap \mn{ok}_{n-1} \sqcap \overline{A}_i \sqcap \exists R . V'
  \sqcap A_\sigma \sqcap A'_{q,\sigma'} &\sqsubseteq& V'_{L,\sigma} \\[1mm]
  % \mn{ok}_0 \sqcap  \cdots \sqcap \mn{ok}_{n-1} \sqcap \overline{A}_i \sqcap \exists R . V'
  % \sqcap A_{q,\sigma} \sqcap A'_{\sigma'} &\sqsubseteq& V'_{R,q} \\[1mm]
  % \mn{ok}_0 \sqcap  \cdots \sqcap \mn{ok}_{n-1} \sqcap \overline{A}_i \sqcap \exists R . V_{L,\sigma}
  % \sqcap A_{q},\sigma'} \sqcap A'_{\sigma''} &\sqsubseteq& V'_{L,q,\sigma} \\[1mm]
  \mn{ok}_0 \sqcap  \cdots \sqcap \mn{ok}_{n-1} \sqcap \overline{A}_i \sqcap \exists R . V_{R,q}
  \sqcap A_{\sigma} \sqcap A'_{q',\sigma'} &\sqsubseteq& V'_{R,q,\sigma} \\[1mm]
  \mn{ok}_0 \sqcap  \cdots \sqcap \mn{ok}_{n-1} \sqcap \overline{A}_i \sqcap \exists R . V'_{M,q,\sigma}
  \sqcap A_{\sigma'} \sqcap A'_{\sigma'} &\sqsubseteq& V'_{M,q,\sigma}
\end{array}
$$
where $\sigma,\sigma',\sigma''$ range over $\Gamma$, $q$ and $q'$ over
$Q$, and $i$ over $0..n-1$. We switch to different verification
markers $V'$, $V'_{L,\sigma}$, $V'_{R,q}$, $V'_{M,q,\sigma}$ to
distinguish halting from non-halting configurations. Note that the
first verification step is different for the latter: we expect to see
one successor marked $X_L$ and one marked $X_R$, both the first cell of an
already verified (halting or non-halting) configuration. For easier
construction, we require two successors also for existential
configurations; they can simply be identical.  The above inclusions do
not yet deal with cells where the head is currently located. We need
some prerequisites because when verifying these cells, we want to
(locally) verify the transition relation. For this purpose, we carry
the transitions implemented locally at a configuration up to its
predecessor configuration:
$$
\begin{array}{r@{~}c@{~}l}
  % A_{q_1,\sigma_1} \sqcap \exists r . (A'_{q_2,\sigma_2} \sqcap A_{\sigma_3}) &\sqsubseteq&
  % S_{q_1,\sigma_3,L} \\[1mm]
  % A'_{q_1,\sigma_1}  \sqcap A_{\sigma_2} \sqcap \exists r . A_{q_2,\sigma_3} &\sqsubseteq&
  % S_{q_2,\sigma_2,R} \\[1mm]
  % \overline{A}_i \sqcap \exists r . S_{q,\sigma,M} &\sqsubseteq& S_{q,\sigma,M}
  % \\[1mm]
  \exists R . \exists R . (X_M \sqcap \overline{A}_0 \sqcap \cdots \sqcap
  \overline{A}_{n-1} \sqcap  V_{q,\sigma,M'}) & \sqsubseteq&
  S^M_{q,\sigma,M'} \\[1mm]
  \exists R . \exists R . (X_M \sqcap \overline{A}_0 \sqcap \cdots \sqcap
  \overline{A}_{n-1} \sqcap  V'_{q,\sigma,M'}) & \sqsubseteq&
  S^M_{q,\sigma,M'} \\[1mm]
  \exists R . (A_{\sigma} \sqcap S^M_{q,\sigma',M}) &\sqsubseteq&
  S^M_{q,\sigma',M} \\[1mm]
\end{array}
$$
where $q$ ranges over $Q$, $\sigma$ and $\sigma'$ over $\Gamma$, $M$
over $\{L,R\}$, and $i$ over $0..n-1$.  Note that markers are
propagated up exactly to the head position. One issue with the above
is that additional $S_{q\sigma,M}$-markers could be propagated up not
from the successors that we have verified, but from surplus
(unverified) successors. To prevent such undesired markers, we put
$$
S^M_{q_1,\sigma_1,M_1} \sqcap S^M_{q_2,\sigma_2,M_2} \sqsubseteq \bot
$$
for all $M \in \{L,R\}$ and all distinct
$(q_1,\sigma_1,M_1),(q_2,\sigma_2,M_2) \in Q \times \Gamma \times
\{L,R\}$.  We can now implement the verification of cells under the
head in non-halting configurations. Put
$$
\begin{array}{rcl}
  \mn{ok}_0 \sqcap  \cdots \sqcap \mn{ok}_{n-1} \sqcap \overline{A}_i \sqcap \exists R . V'
  \sqcap
  A_{q_1,\sigma_1} \sqcap A'_{\sigma_1} \sqcap S^L_{q_2,\sigma_2,M_2}
  \sqcap S^R_{q_3,\sigma_3,M_3}&\sqsubseteq& V'_{R,q_1} \\[2mm]
  \mn{ok}_0 \sqcap  \cdots \sqcap \mn{ok}_{n-1} \sqcap \overline{A}_i \sqcap \exists R . V'_{L,\sigma}
  \sqcap
  A_{q_1,\sigma_1} \sqcap A'_{\sigma_1} \sqcap S^L_{q_2,\sigma_2,M_2}
  \sqcap S^R_{q_3,\sigma_3,M_3}&\sqsubseteq& V'_{L,q_1,\sigma}
\end{array}
$$
for all $(q_1,\sigma_1) \in Q \times \Gamma$ with $q_1$ a universal
state and
$\Delta(q_1,\sigma_1)=\{(q_2,\sigma_2,M_2),(q_3,\sigma_3,M_3)\}$, $i$
from $0..n-1$, and $\sigma$ from $\Gamma$; moreover, put
$$
\begin{array}{rcl}
   \mn{ok}_0 \sqcap  \cdots \sqcap \mn{ok}_{n-1} \sqcap \overline{A}_i \sqcap \exists R . V'
   \sqcap
   A_{q_1,\sigma_1} \sqcap A'_{\sigma_1} \sqcap S^L_{q_2,\sigma_2,M_2}
   \sqcap S^R_{q_2,\sigma_2,M_2}&\sqsubseteq& V'_{R,q_1} \\[2mm]
   \mn{ok}_0 \sqcap  \cdots \sqcap \mn{ok}_{n-1} \sqcap \overline{A}_i \sqcap \exists R . V'_{L,\sigma}
   \sqcap
   A_{q_1,\sigma_1} \sqcap A'_{\sigma_1} \sqcap S^L_{q_2,\sigma_2,M_2}
   \sqcap S^R_{q_2,\sigma_2,M_2}&\sqsubseteq& V'_{L,q,\sigma}
\end{array}
$$
for all $(q_1,\sigma_1) \in Q \times \Gamma$ with $q_1$ an existential
state, for all $(q_2,\sigma_2,M_2) \in \Delta(q_1,\sigma_1)$, all $i$
from $0..n-1$, and all $\sigma$ from~$\Gamma$.  It remains to verify
the initial configuration. Let $w=\sigma_0 \cdots \sigma_{n-1}$, let
$(C=i)$ be the conjunction over the concept names $A_i$,
$\overline{A}_i$ that expresses $i$ in binary for $0 \leq i < n$, and
let $(C \geq n)$ be the Boolean concept over the concept names $A_i$,
$\overline{A}_i$ which expresses that the counter value is at least
$n$. Then put
$$
\begin{array}{r@{\,}c@{\,}l}
  A_0 \sqcap \cdots \sqcap A_{n-1} \sqcap A_\Box \sqcap A'_\sigma
  \sqcap L\mn{ok} \sqcap R\mn{ok}   &\sqsubseteq& V^I \\[1mm]
\mn{ok}_0 \sqcap  \cdots \sqcap \mn{ok}_{n-1}
\sqcap (C \geq n) \sqcap \exists R . V^I
  \sqcap A_\Box \sqcap A'_\sigma &\sqsubseteq& V^I \\[1mm]
 \mn{ok}_0 \sqcap  \cdots \sqcap \mn{ok}_{n-1} \sqcap (C=i) \sqcap \exists R . V^I
  \sqcap A_{\sigma_i}\sqcap A'_\sigma &\sqsubseteq& V^I \\[1mm]
 \mn{ok}_0 \sqcap  \cdots \sqcap \mn{ok}_{n-1} \sqcap (C=1) \sqcap \exists R . V^I
  \sqcap A_{\sigma_1}\sqcap A'_{q,\sigma'} &\sqsubseteq& V^I_{R,q}
\end{array}
$$
where $i$ ranges over $2..n-1$ and $\sigma,\sigma'$ over $\Gamma$.  This
verifies the initial conditions except for the left-most cell, where the head
must be located (in initial state $q_0$) and where we must verify the
transition, as in all other configurations.  Recall that we assume
$q_0$ to be an existential state. We can thus add
$$
\begin{array}{rcl}
   \mn{ok}_0 \sqcap  \cdots \sqcap \mn{ok}_{n-1} \sqcap (C=0) \sqcap \exists R . V^I_{R,q}
   \sqcap
   A_{q_0,\sigma_0} \sqcap A'_\sigma \sqcap S^L_{q,\sigma,M}
   \sqcap S^R_{q,\sigma,M}&\sqsubseteq& I
\end{array}
$$
for all $(q,\sigma,M) \in \Delta(q_0,\sigma_0)$ and $\sigma \in \Gamma$.

At this point, we have finished the verification of the computation
tree, except that we have assumed but not yet established ($*$). To
achieve ($*$), we use both $\Tmc_1$ and $\Tmc_2$. Let
$\alpha_0,\dots,\alpha_{k-1}$ be the elements of $\Gamma \cup (Q
\times \Gamma)$. We use concept names $A^\ell_i$,
$\overline{A}^\ell_i$, $\ell \in \{0,\dots,k-1\}$, to implement $k$
additional counters. This time, we have to count up to $2^n+1$
(because successor configuration sequences are separated by two
edges), so $i$ ranges from $0$ to $m := \lceil \mn{log}(2^n+1)
\rceil$.  We first add to $\Tmc_2$:
$$
\begin{array}{rcl}
  \exists R . I & \sqsubseteq & \exists S .  \midsqcap_{\ell <k}
  \exists R . (A_{\alpha_\ell} \sqcap (C^\ell = 0)) \\[1mm]
  \overline{A}^\ell_i &\sqsubseteq& \exists R . \top \\[1mm]
  A^\ell_i \sqcap \midsqcap_{j < i} A^\ell_j & \sqsubseteq& \forall R
  . \overline{A}^\ell_i \\[1mm]
  \overline{A}^\ell_i \sqcap \midsqcap_{j < i} A^\ell_j & \sqsubseteq& \forall R
  . A^\ell_i \\[1mm]
  A^\ell_i \sqcap \midsqcup_{j < i} \overline{A}^\ell_j & \sqsubseteq& \forall R
  . A^\ell_i \\[1mm]
  \overline{A}^\ell_i \sqcap \midsqcup_{j < i} \overline{A}^\ell_j & \sqsubseteq& \forall R
  . \overline{A}^\ell_i \\[1mm]
  (C^\ell = 2^n) & \sqsubseteq & \overline{A}_{\alpha_\ell}
\end{array}
$$
where $\ell$ ranges over $0..k-1$, $i$ over $0..m-1$, and $(C^\ell = j)$
denotes the conjunction over $A^\ell_i$, $\overline{A}^\ell_i$ which
expresses that the value of the $\ell$-th counter is $j$.  We will
explain shortly why we need to travel one more $R$-step (in the first
line) after seeing~$I$.

The above inclusions generate, after the verification of the
computation tree has ended successfully, a tree in the canonical model
of the input ABox and of $\Tmc_2$ as shown in Figure~\ref{fig:mod}.
\begin{figure}[t!]
  \begin{center}
    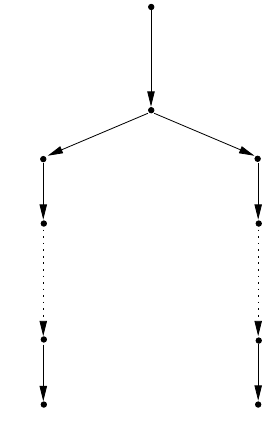
    \caption{Tree gadget.}
    \label{fig:mod}
  \end{center}
\end{figure}
Note that the topmost edge is labeled with the role name $S$, which is
\emph{not} in~$\Sigma$. By Condition~(b) above and since, up to now,
we have always only used non$-\Sigma$-symbols on the right-hand side
of concept inclusions, we must not (homomorphically) find the subtree
rooted at the node with the incoming $S$-edge \emph{anywhere} in the
canonical model of the ABox and $\Tmc_1$. We use this effect which we
to ensure that ($*$) is satisfied \emph{everywhere}. Note that, the
paths in Figure~\ref{fig:mod} have length $2^n+1$ and that we do not
display the labeling with the concept names $A^\ell_i$,
$\overline{A}^\ell_i$.  These concept names are not in $\Sigma$ anyway
and only serve the purpose of achieving the intended path
length. Intuitively, every path in the tree represents one possible
\emph{copying defect}. The concept names of the form
$\overline{A}_\alpha$ need not occur in the input ABox and
stand for the disjunction over all $\overline{A}_\beta$ with $\beta
\neq \alpha$. They need to be in $\Sigma$, though, because we want
them to be taken into account in $\Sigma$-homomorphisms.

\smallskip

We
next extend $\Tmc_1$ as follows:
$$
\begin{array}{rcl}
  A_{\alpha} &\sqsubseteq& \overline{A}_\beta \\[1mm]
  \exists R . A_{\alpha_i} & \sqsubseteq& \midsqcap_{\ell \in \{0,\dots,k-1\}
    \setminus \{i\}} \exists R . (A_{\alpha_\ell} \sqcap
(C^\ell=0)) \\[1mm]
  \overline{A}^\ell_i &\sqsubseteq& \exists R . \top \\[1mm]
  A^\ell_i \sqcap \midsqcap_{j < i} A^\ell_j & \sqsubseteq& \forall R
  . \overline{A}^\ell_i \\[1mm]
  \overline{A}^\ell_i \sqcap \midsqcap_{j < i} A^\ell_j & \sqsubseteq& \forall R
  . A^\ell_i \\[1mm]
  A^\ell_i \sqcap \midsqcup_{j < i} \overline{A}^\ell_j & \sqsubseteq& \forall R
  . A^\ell_i \\[1mm]
  \overline{A}^\ell_i \sqcap \midsqcup_{j < i} \overline{A}^\ell_j & \sqsubseteq& \forall R
  . \overline{A}^\ell_i \\[1mm]
  (C^\ell = 2^n) & \sqsubseteq & \overline{A}_{\alpha_\ell}
\end{array}
$$
where $\ell$ ranges over $0..k-1$, $i$ over $0..m-1$, and
$\alpha,\beta$ over distinct elements of $\Gamma \cup (Q\times
\Gamma)$. Note that it is not important to use the same counter
concepts $A^\ell_i$, $\overline{A}^\ell_i$ in $\Tmc_1$ and $\Tmc_2$:
since they are not in $\Sigma$, one could as well use different ones.
Also note that the intended behaviour of the concept names
$\overline{A}_\alpha$ is implemented in the first line.

\smallskip

The idea for achieving ($*$) is as follows: the tree shown in
Figure~\ref{fig:mod} contains all possible copying defects, that is,
all paths of length $2^n+1$ such that $A_{\alpha_i}$ is true at the
beginning, but some $A_{\alpha_j}$ with $j \neq i$ is true at the end.
At each point of the computation tree where some $A_{\alpha_i}$ is
true at an $R$-predecessor, the above inclusions in $\Tmc_1$ generate
a tree in the canonical model of the ABox and of $\Tmc_1$ which is
similar to that in Figure~\ref{fig:mod}, except that the initial
$S$-edge and the path representing an $A_{\alpha_i}$-defect are
missing. Consequently, if $A_{\alpha_i}$ is not properly copied to
$A'_{\alpha_i}$ at all nodes that are $2^n+1$ $R$-steps away, then we
homomorphically find the tree from Figure~\ref{fig:mod} in the
canonical model of the ABox and of $\Tmc_1$. Consequently, not finding
the tree anywhere in that model means that all copying is done
correctly.

We need to avoid that the inclusions in $\Tmc_1$ enable a homomorphism
from the tree in Figure~\ref{fig:mod} due to an ABox where some node
has two $R$-successors labeled with different concepts $A_\alpha$,
$A_\beta$:
$$
  \exists R. A_\alpha \sqcap \exists R . A_\beta \sqsubseteq \bot.
$$
This explains why we need to separate successor configurations by two
$R$-steps. In fact, the mid point needs not make true any of the
concept names $A_\alpha$ and thus we are not forced to violate the
above constraint when branching at the end of configuration
sequences. Also note that copying the content of the first cell of the
initial configuration requires traveling one more $R$-step after
seeing $I$, as implemented above.
\begin{lemma}
\label{lem:2expcorr}
  The following conditions are equivalent:
\begin{enumerate}

\item there is a tree-shaped $\Sigma$-ABox \Amc\xspace such that
  \begin{enumerate}
  \item \Amc is consistent w.r.t.\ $\Tmc_1$ and $\Tmc_2$ and

  \item $\Imc_{\Tmc_2,\Amc}$ is not
    $\Sigma$-homomorphically embeddable into
    $\Imc_{\Tmc_1,\Amc}$;

  \end{enumerate}

\item $M$ accepts $w$.

\end{enumerate}
\end{lemma}
\begin{proof}(sketch) For the direction ``$2 \Rightarrow 1$'', assume
  that $M$ accepts $w$. An accepting computation tree of $M$ on $w$
  can be represented as a $\Sigma$-ABox as detailed above alongside
  the construction of the TBoxes $\Tmc_2$ and $\Tmc_1$. The
  representation only uses the role name $R$ and the concept names of
  the form $A_i$, $\overline{A}_i$, $A_\sigma$, $A_{q,\sigma}$,
  $A'_\sigma$, $A'_{q,\sigma}$, $X_L$, and $X_R$, but not the concept
  names of the form $\overline{A}_\sigma$ and
  $\overline{A}_{q,\sigma}$. As explained above, we need to duplicate
  the successor configurations of existential configurations to ensure
  that there is binary branching after each configuration. Also, we
  need to add one additional incoming $R$-edge to the root of the tree
  as explained above. The resulting ABox \Amc is consistent w.r.t.\
  $\Tmc_1$ and $\Tmc_2$. Moreover, since there are no copying defects,
  there is no homomorphism from $\Imc_{\Tmc_2,\Amc}$ to
  $\Imc_{\Tmc_1,\Amc}$.

  \smallskip

  For the direction ``$1 \Rightarrow 2$'', assume that there is a
  tree-shaped $\Sigma$-ABox \Amc that satisfies Conditions~(a)
  and~(b).  Because of Condition~(b), $I$ must be true somewhere in
  $\Imc_{\Tmc_2,\Amc}$: otherwise, $\Imc_{\Tmc_2,\Amc}$ does not
  contain anonymous elements and the identity is a homomorphism from
  $\Imc_{\Tmc_2,\Amc}$ to $\Imc_{\Tmc_1,\Amc}$, contradicting
  (b). Since $I$ is true somewhere in $\Imc_{\Tmc_2,\Amc}$ and by
  construction of $\Tmc_2$, the ABox must contain the representation
  of a computation tree of $M$ on $w$, except satisfaction of ($*$).
  For the same reason, $\Imc_{\Tmc_2,\Amc}$ must contain a tree as
  shown in Figure~\ref{fig:mod}.  As has already been argued during
  the construction of $\Tmc_2$ and $\Tmc_1$, however, condition ($*$)
  follows from the existence of such a tree in $\Imc_{\Tmc_2,\Amc}$
  together with (b).
\end{proof}
We remark that the above reduction also yields 2\ExpTime hardness for
CQ entailment in $\mathcal{ELI}$. In fact, universal restrictions on
the right-hand sides of concept inclusions can easily be simulated
using universal roles and disjunctions on the left-hand sides can be
removed with only a polynomial blowup (since there are always only two
disjuncts). It thus remains to eliminate $\bot$, which only occurs
non-nested on the right-hand side of concept inclusions. With the
exception of the inclusions
$$
S^M_{q_1,\sigma_1,M_1} \sqcap S^M_{q_2,\sigma_2,M_2} \sqsubseteq \bot,
$$
this can be done as follows: include all concept inclusions with
$\bot$ on the right-hand side in $\Tmc_1$ instead of in $\Tmc_2$; then
replace $\bot$ with $D$ and add the following concept inclusions to
$\Tmc_1$:
$$
\begin{array}{rcl}
  D& \sqsubseteq & \exists S .  \midsqcap_{\ell <k}
  \exists R . (A_{\alpha_\ell} \sqcap (C^\ell = 0)) \\[1mm]
  \overline{A}^\ell_i &\sqsubseteq& \exists R . \top \\[1mm]
  A^\ell_i \sqcap \midsqcap_{j < i} A^\ell_j & \sqsubseteq& \forall R
  . \overline{A}^\ell_i \\[1mm]
  \overline{A}^\ell_i \sqcap \midsqcap_{j < i} A^\ell_j & \sqsubseteq& \forall R
  . A^\ell_i \\[1mm]
  A^\ell_i \sqcap \midsqcup_{j < i} \overline{A}^\ell_j & \sqsubseteq& \forall R
  . A^\ell_i \\[1mm]
  \overline{A}^\ell_i \sqcap \midsqcup_{j < i} \overline{A}^\ell_j & \sqsubseteq& \forall R
  . \overline{A}^\ell_i \\[1mm]
  (C^\ell = 2^n) & \sqsubseteq & \overline{A}_{\alpha_\ell}
\end{array}
$$
where $\ell$ ranges over $0..k-1$ and $i$ over $0..m$.  The effect of
these additions is that any ABox which satisfies the left-hand side of
a $\bot$-concept inclusion in the original $\Tmc_2$ cannot satisfy
Condition~(b) from Lemma~\ref{lem:2expcorr} and thus needs not be
considered.

For the inclusions excluded above, a different approach needs to be
taken. Instead of introducing the concept names
$S^M_{q_1,\sigma_1,M_1}$, one would propagate transitions inside the
$V'$-markers. Thus, $S^{L}_{q_1,\sigma_1,M_1}$,
$S^R_{q_2,\sigma_2,M_2}$, and $V'$ would be integrated into a single
marker $V'_{q_1,\sigma_1,M_1,q_2,\sigma_2,M_2}$, and likewise for
$V_{R,q}$. The concept inclusion excluded above can then simply be
dropped.

\endinput

%%% Local Variables:
%%% mode: latex
%%% TeX-master: "aij-insep"
%%% TeX-PDF-mode: t
%%% fill-column: 79
%%% save-place: t
%%% End:
